# Supplementary material for: FisheyeDistanceNet: Self-Supervised Scale-Aware Distance Estimation using Monocular Fisheye Camera for Autonomous Driving
Source: arXiv:1910.04076 source file (2020-10-06)
Supplement: Supplementary file 1 [file fisheye.tex]

\section{Overview of Fisheye Camera Projections} 
\label{sec:fisheye}

Fisheye cameras exhibit significantly more complex projection geometry and the images display severe distortion. Typical camera datasets like KITTI~\cite{geiger2013vision} and CityScapes~\cite{cordts2016cityscapes} consist of relatively narrow FOV camera data where a simple pinhole projection model is commonly employed. In case of fisheye camera images, it is imperative that the appropriate camera model is well understood either to handle distortion in the algorithm or to warp the image prior to processing. This section is intended to highlight to the reader that the fisheye camera model requires specific attention. We provide a brief overview and references for further details, and discuss the merits of operating on the raw fisheye versus undistortion of the image.

Fisheye distortion is modeled by a radial mapping function $r(\theta)$, where $r(\theta)$ is the distance on the image from the centre of distortion, and is a function of the angle $\theta$ of the incident ray against the optical axis of the camera system. The centre of distortion is the intersection of the optical axis with the image plane, and is the origin of the radial mapping function $r(\theta)$. Stereographic projection \cite{herbert1987area} is the simplest model which uses a mapping from a sphere to a plane. More recent projection models are Unified Camera Model (UCM) \cite{barreto2006unified, caruso2015large} and eUCM (Enhanced UCM) \cite{Khomutenko2016eucm}. More detailed analysis of accuracy of various
rojection models is discussed in \cite{hughes2010fisheye}. These models are not a perfect fit for fisheye cameras as they encode a specific geometry (e.g. spherical projection), and errors arising in the model are compensated by using an added distortion correction component. %, typically in the form of an odd ordered polynomial mapping from distorted image to undistorted image. 

We use model parameters for a more generic fisheye intrinsic calibration that is independent of any specific projection model and does not require the added step of distortion correction. Our model is based on a fourth order polynomial mapping incident angle to image radius in pixels ($r(\theta) = a_1 \theta + a_2 \theta^2 + a_3 \theta^3 + a_4 \theta^4$).
In our experience, higher orders provide no additional accuracy.

The inverse of $r(\theta)$ for the $4^\text{th}$ order polynomial requires root solving, which can be expensive (albeit, this can be overcome by the use of a look-up table for the inverse as we are certain that the distortion stays the same throughout the whole dataset. UCM and eUCM, and geometric models in general, are analytically reversible.

\begin{figure}[t!]
    \captionsetup{singlelinecheck=false, justification=raggedright, font=footnotesize, labelsep=space}
    \centering
    \includegraphics[width=0.8\columnwidth]{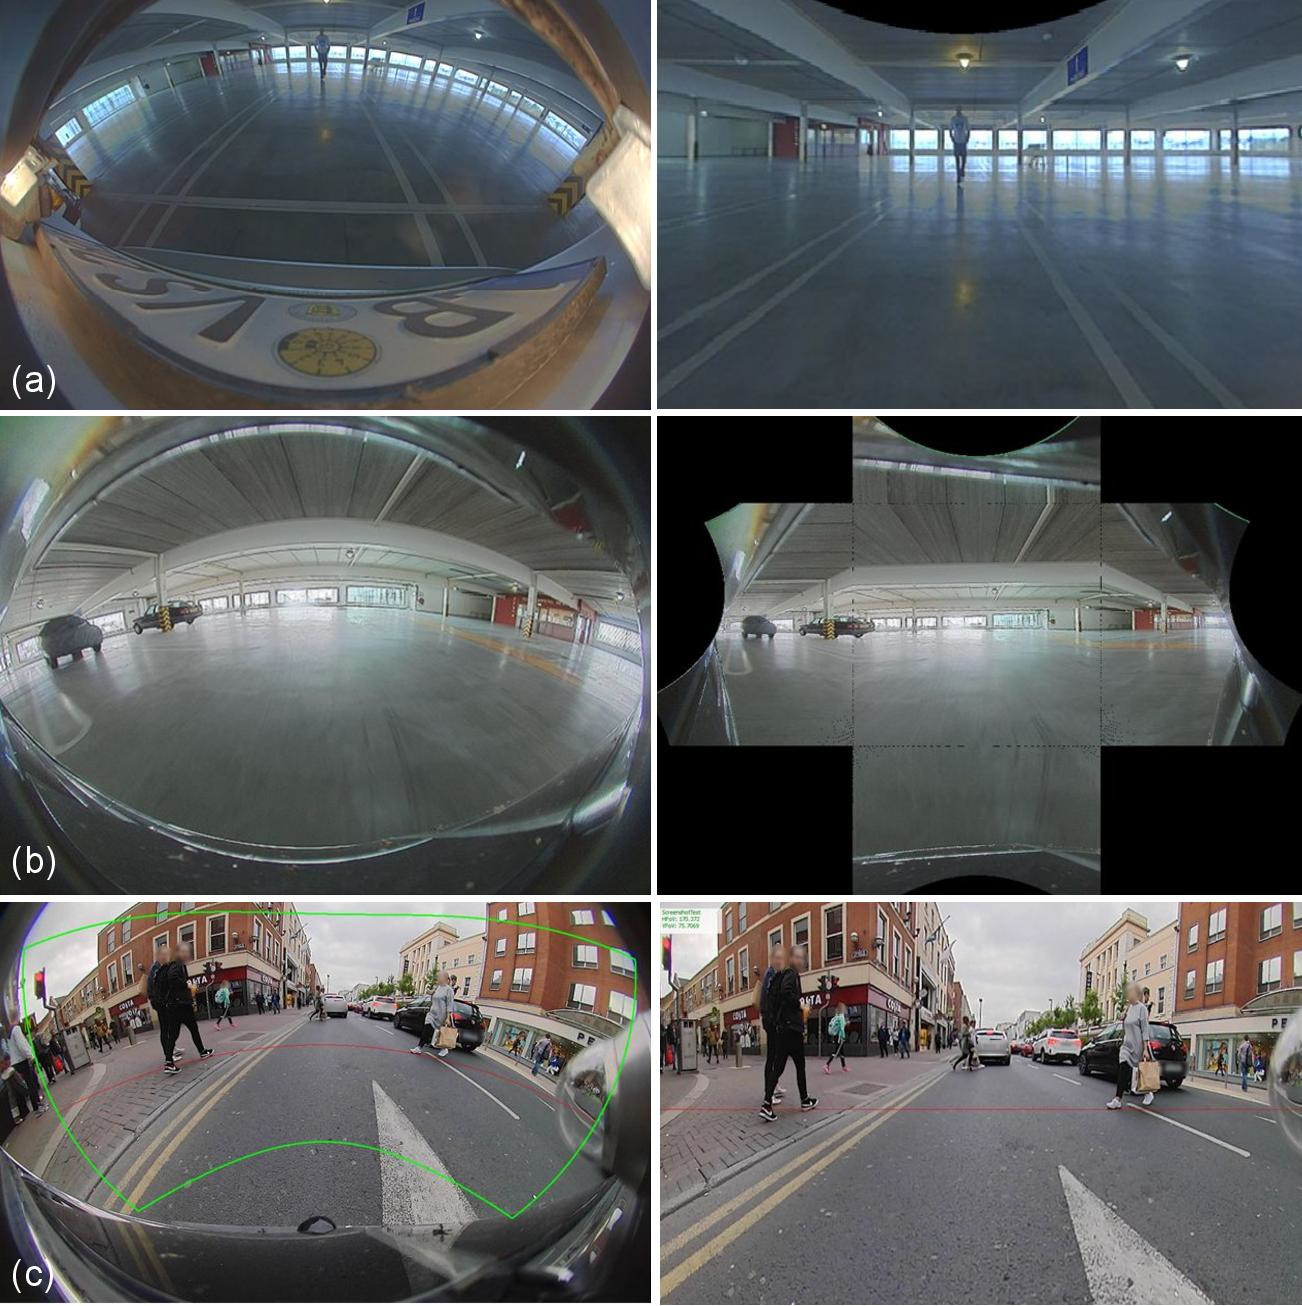}
    \vspace{-0.15cm}
    \caption{Undistorting the fisheye image: 
    (a) Rectilinear correction; (b) Piecewise linear correction; (c) Cylindrical correction. Left: raw image; Right: undistorted image.}\label{fig:projections}
    \vspace{-0.5cm}
\end{figure}

% -------------------------------------------------
\subsection{Image Undistortion vs. Model Adaptation} 
\label{sec:linearization}

Standard computer vision models do not generalize easily to fisheye cameras because of large non-linear distortion. For example, translation invariance is lost for a standard convolutional neural net (CNN). The na\"{i}ve way to develop algorithms for fisheye cameras is to perform rectilinear correction so that standard models can be applied. The simplest undistortion is to re-warp pixels to a rectilinear image as shown in Figure \ref{fig:projections} (a). But there are two major issues. Firstly, the FOV is greater than 180$^\circ$, hence there are rays incident from behind the camera and it is not possible to establish a complete mapping to a rectilinear viewport. This leads to a loss of FOV, this is seen via the missing yellow pillars in the corrected image. Secondly, there is an issue of resampling distortion, which is more pronounced near the periphery of the image where a smaller region gets mapped to a larger region. 

The missing FOV can be resolved by multiple linear viewports as shown in Figure \ref{fig:projections} (b). However there are issues in the transition region from one plane to another. This can be viewed as a piecewise linear approximation of the fisheye lens manifold. Figure \ref{fig:projections} (c) demonstrates a quasi-linear correction using a cylindrical viewport, where it is linear in vertical direction and straight vertical objects like pedestrians are preserved. However, there is a quadratic distortion along the horizontal axis. In many scenarios, it provides a reasonable trade-off but it still has limitations. In case of learning algorithms, a parametric transform can be optimized for optimal performance of the target application accuracy.

Because of fundamental limitations of undistortion, an alternate approach of adapting the algorithm incorporating fisheye projection model discussed in Section~\ref{sec:modeling of fisheye geometry} could be an optimal solution. In case of classical geometric algorithms, an analytical version of non-linear projection can be incorporated. For example, Kukelova et al.~\cite{kukelova2015radial} extend homography estimation by incorporating radial distortion model. In case of deep learning algorithms, a possible solution could be to train the CNN model to learn the distortion. However, the translation invariance assumption of CNN fundamentally breaks down due to spatially variant distortion and thus it is not efficient to let the network learn it implicitly. This had led to several adaptations of CNN to handle spherical images such as \cite{su2018kernel} and \cite{coors2018spherenet}. However, spherical models do not provide an accurate fit for fisheye lenses and it is an open problem.

\begin{figure*}[!ht]
  \captionsetup{singlelinecheck=false, justification=raggedright, font=footnotesize, labelsep=space}
  \centering
  \resizebox{\textwidth}{!}{
  \newcommand{\turnheightnew}{0.25\columnwidth}
\centering

\begin{tabular}{@{\hskip 0.5mm}c@{\hskip 0.5mm}c@{\hskip 0.5mm}c@{\hskip 0.5mm}c@{\hskip 0.5mm}c@{}}

{\rotatebox{90}{\hspace{0mm}Input(cropped)}} &
\includegraphics[height=\turnheightnew]{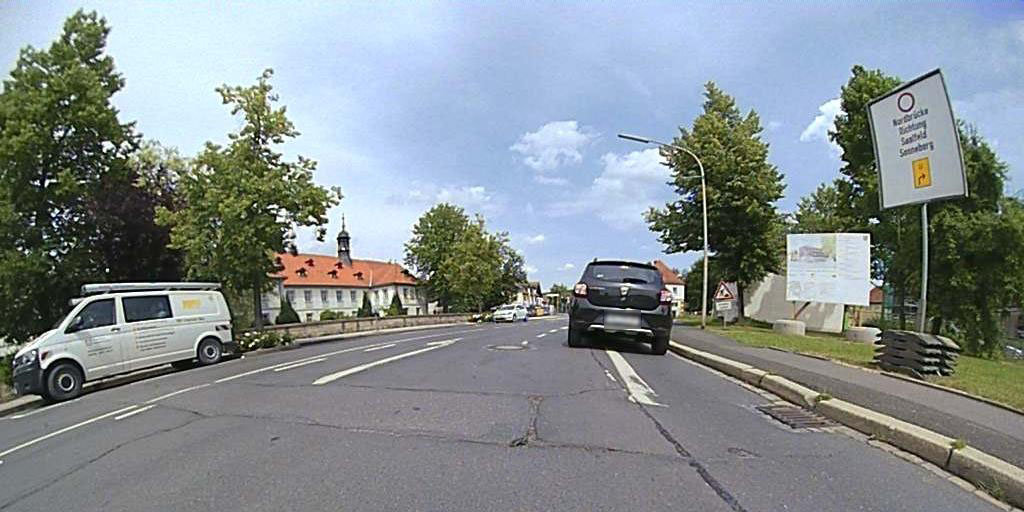} &
\includegraphics[height=\turnheightnew]{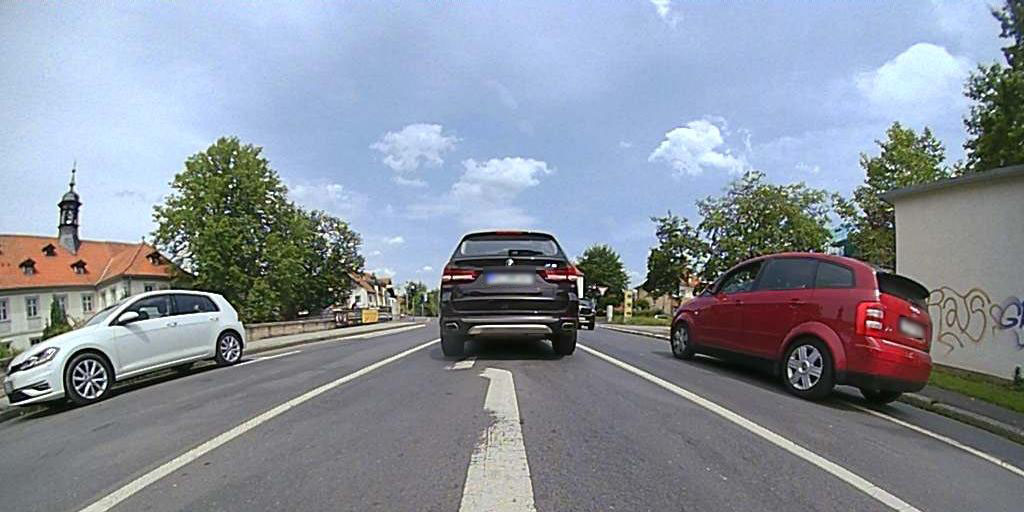} &
\includegraphics[height=\turnheightnew]{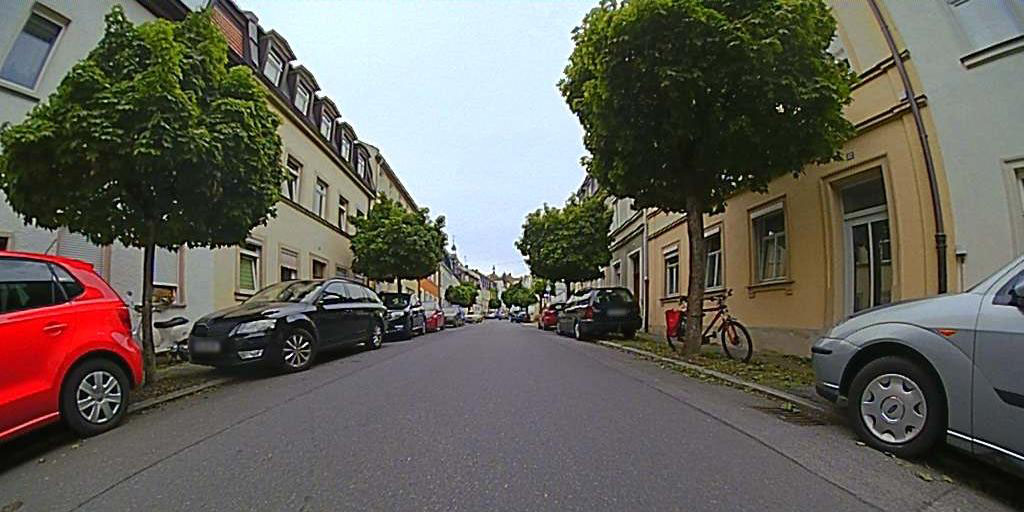} &
\includegraphics[height=\turnheightnew]{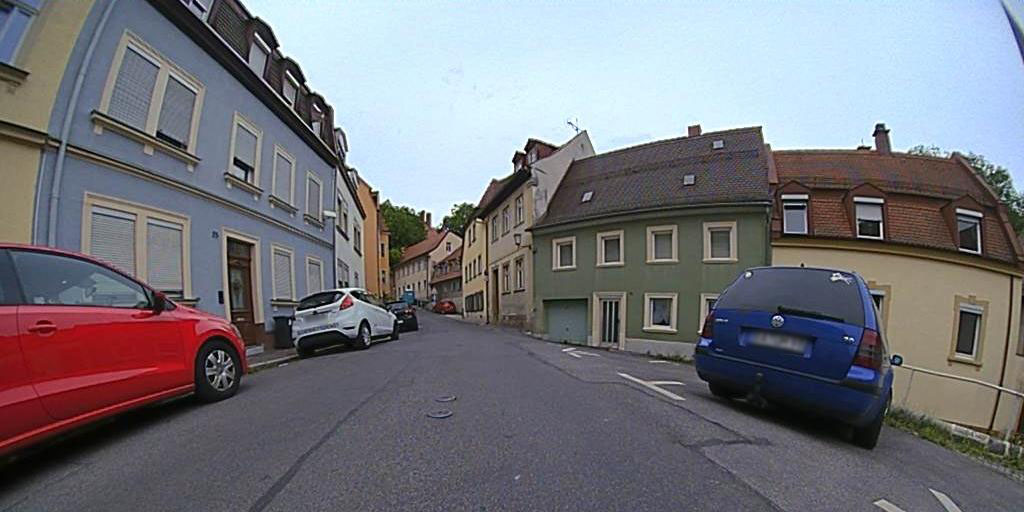}\\

{\rotatebox{90}{\hspace{0mm}}} &
\includegraphics[height=\turnheightnew]{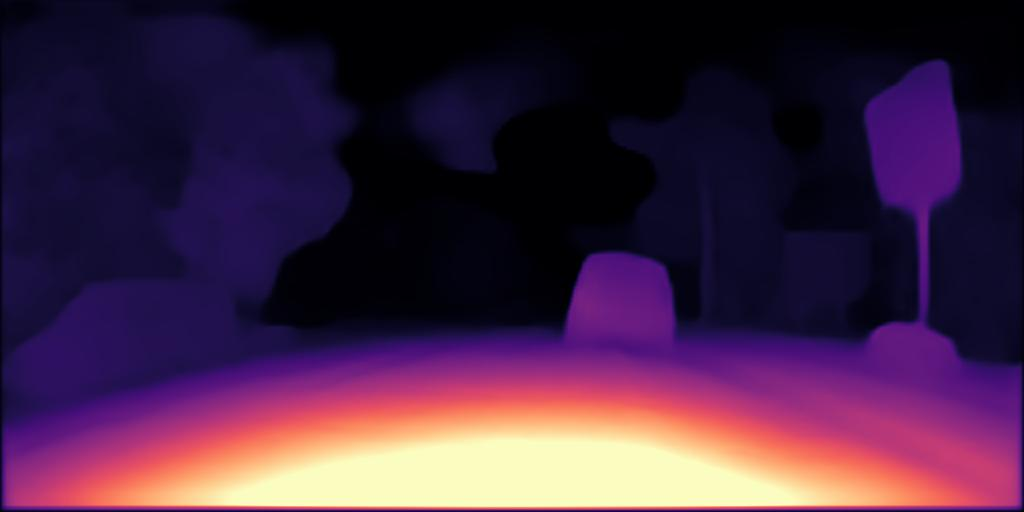} &
\includegraphics[height=\turnheightnew]{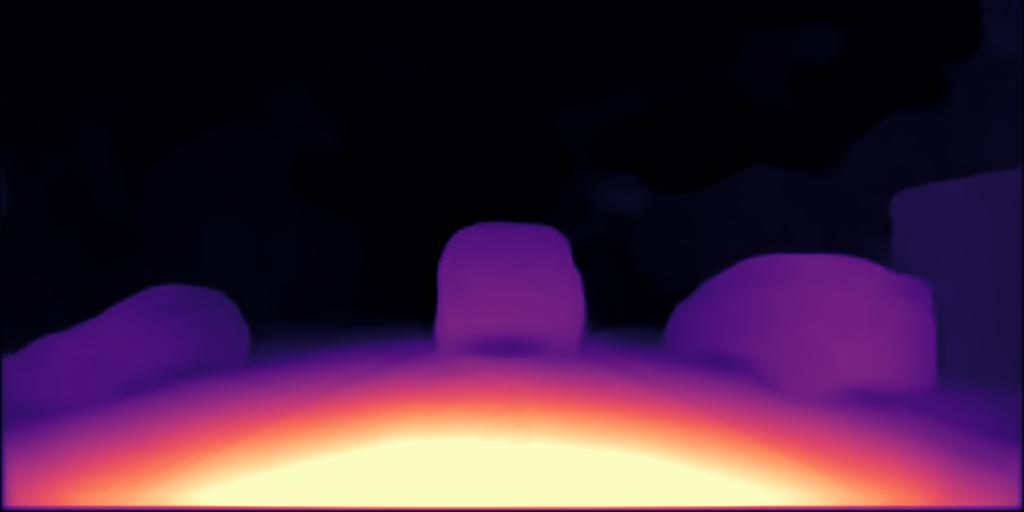} &
\includegraphics[height=\turnheightnew]{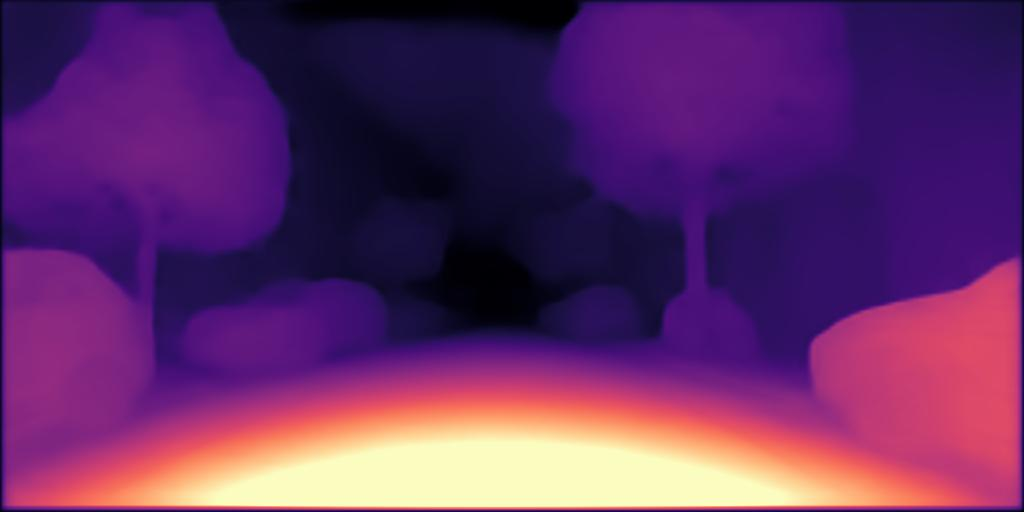} &
\includegraphics[height=\turnheightnew]{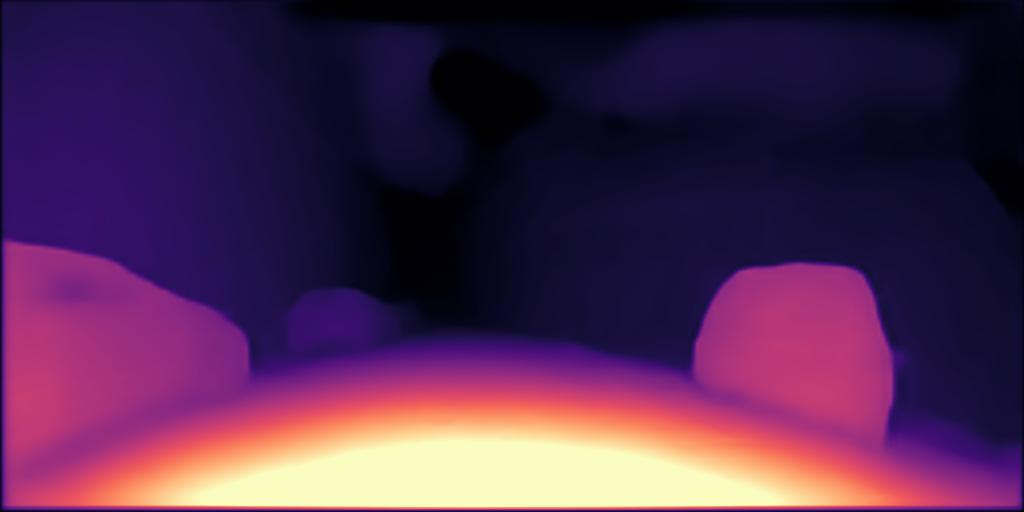}\\

% Distortion
{\rotatebox{90}{\hspace{0mm}\scriptsize}} &
\includegraphics[height=\turnheightnew]{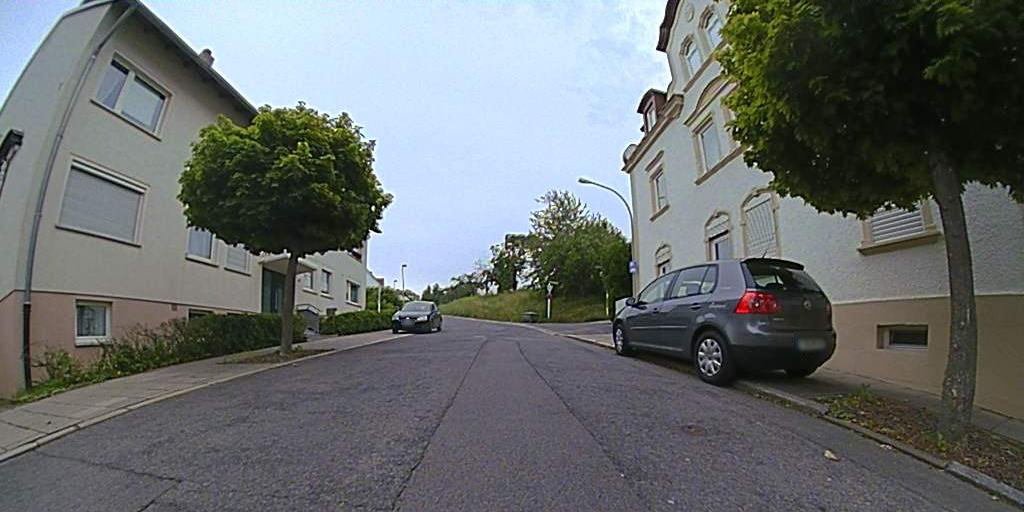} &
\includegraphics[height=\turnheightnew]{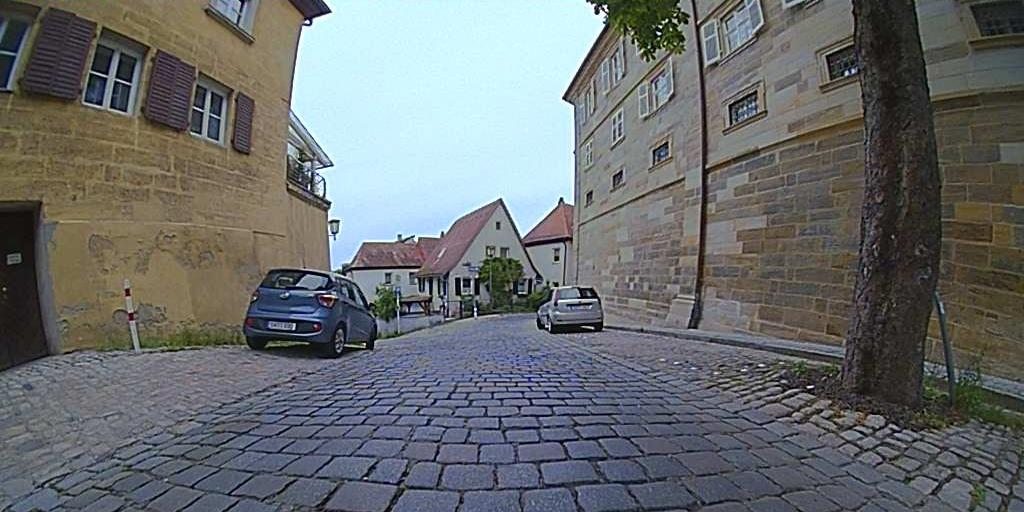} &
\includegraphics[height=\turnheightnew]{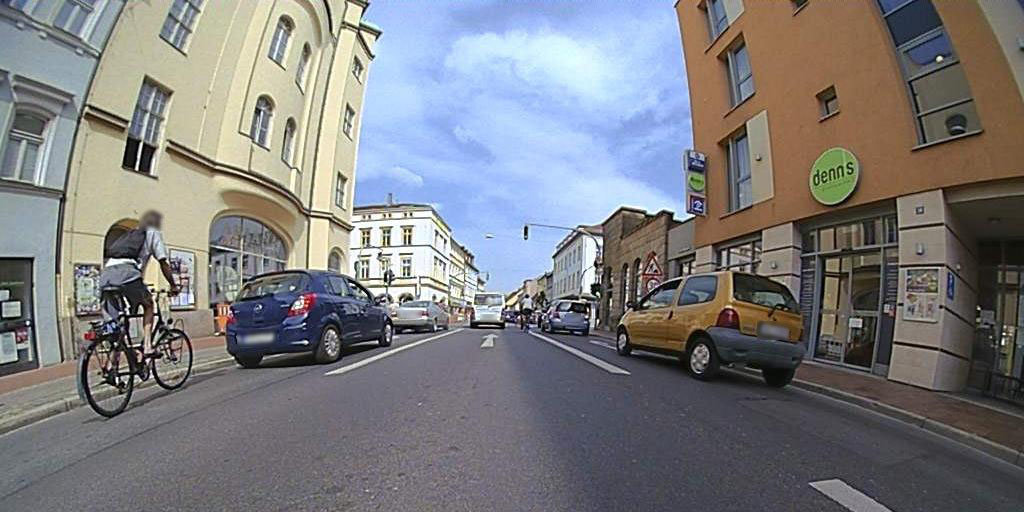} &
\includegraphics[height=\turnheightnew]{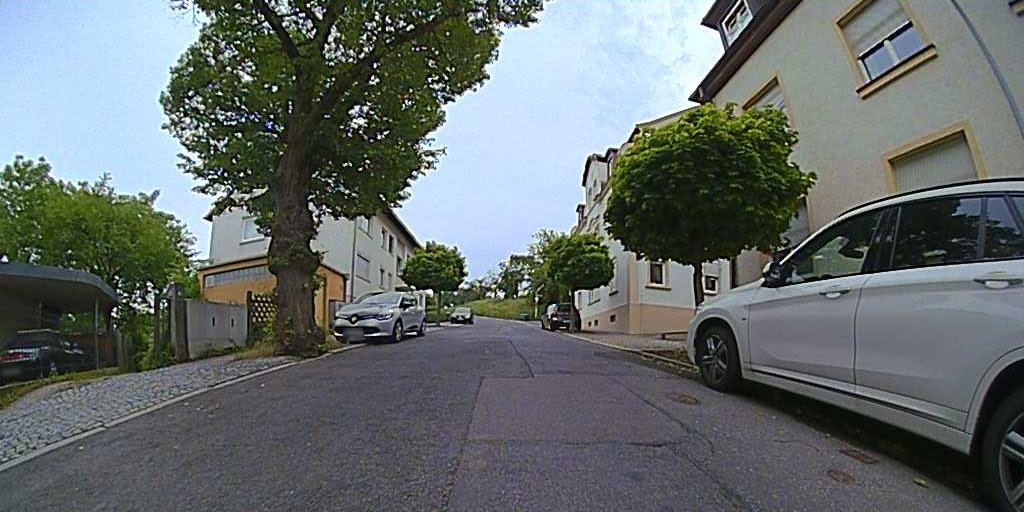} \\

{\rotatebox{90}{\hspace{0mm}\scriptsize}} &
\includegraphics[height=\turnheightnew]{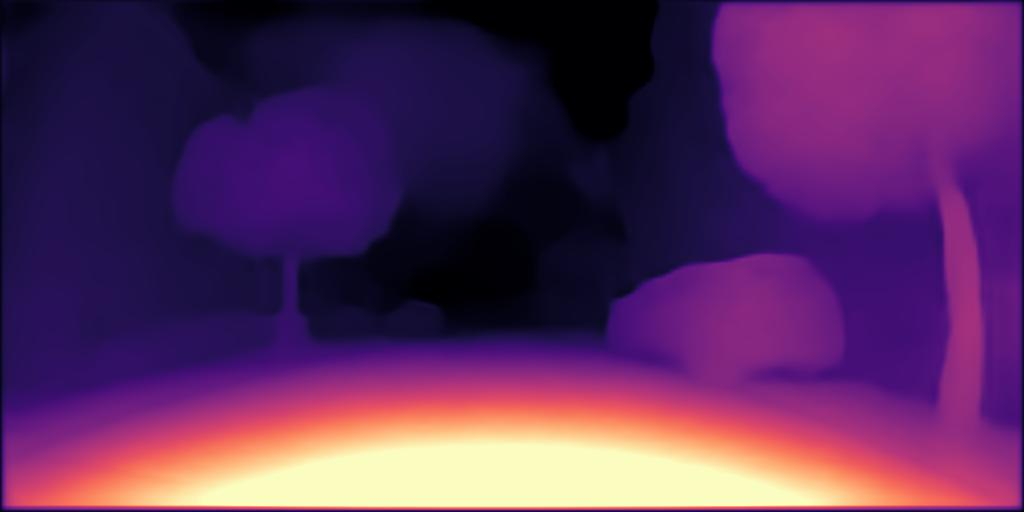} &
\includegraphics[height=\turnheightnew]{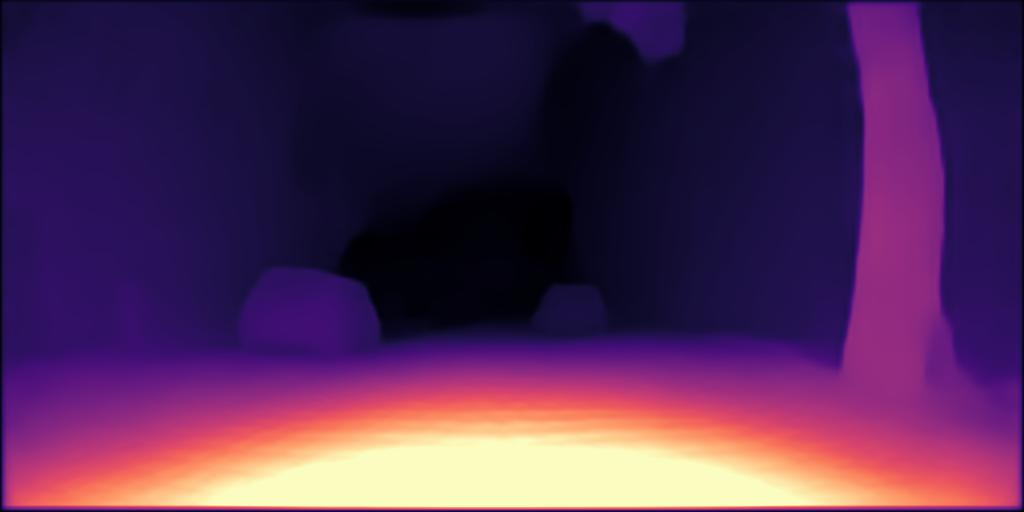} &
\includegraphics[height=\turnheightnew]{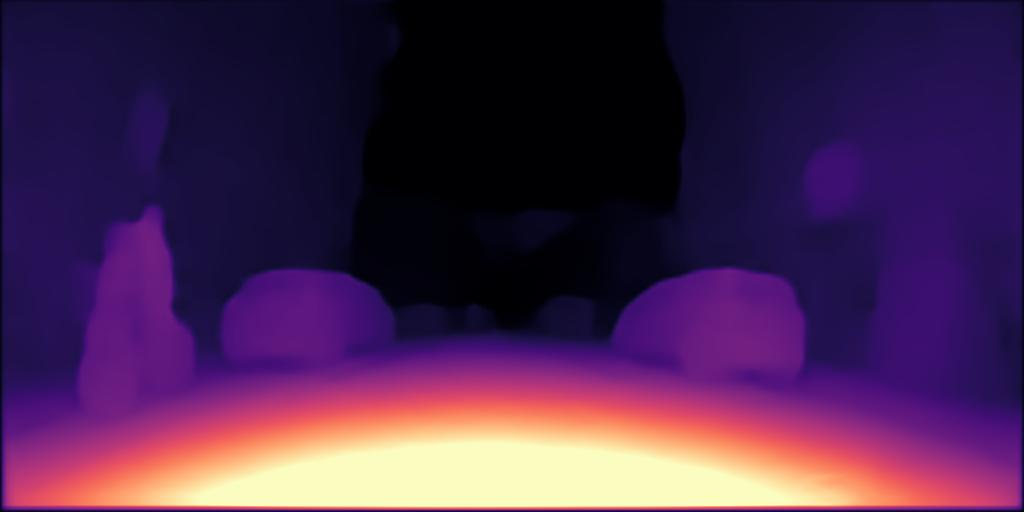} &
\includegraphics[height=\turnheightnew]{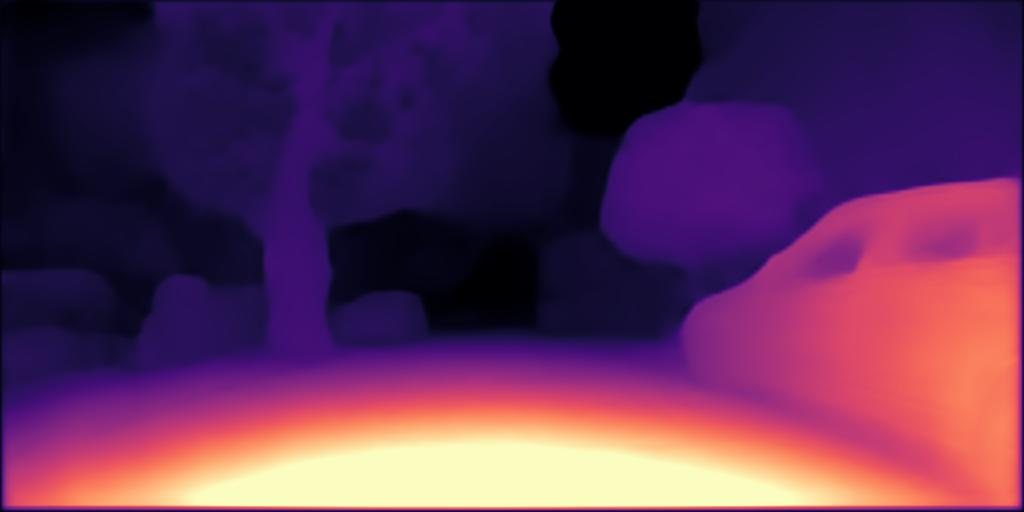} \\

% Sharp Edges
{\rotatebox{90}{\hspace{0mm}\scriptsize}} &
\includegraphics[height=\turnheightnew]{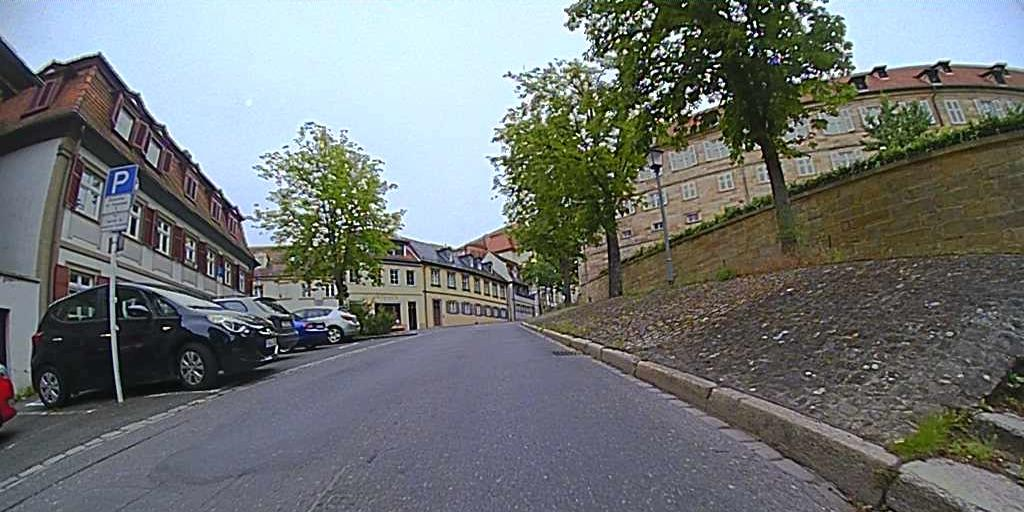} &
\includegraphics[height=\turnheightnew]{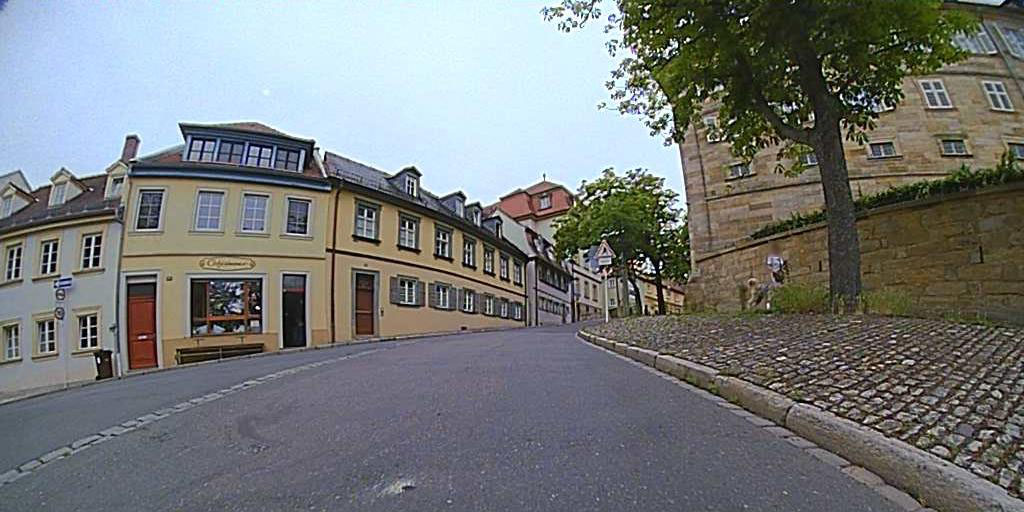} &
\includegraphics[height=\turnheightnew]{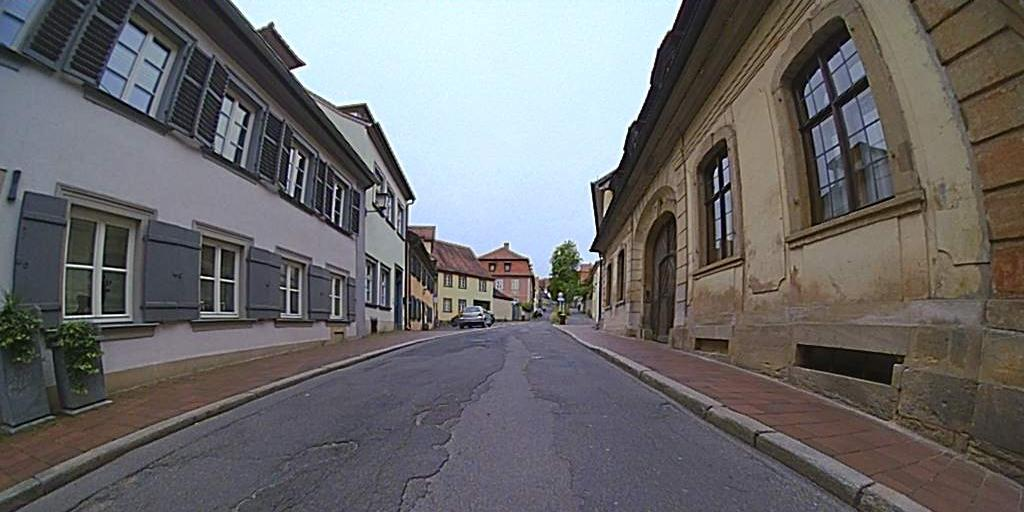} &
\includegraphics[height=\turnheightnew]{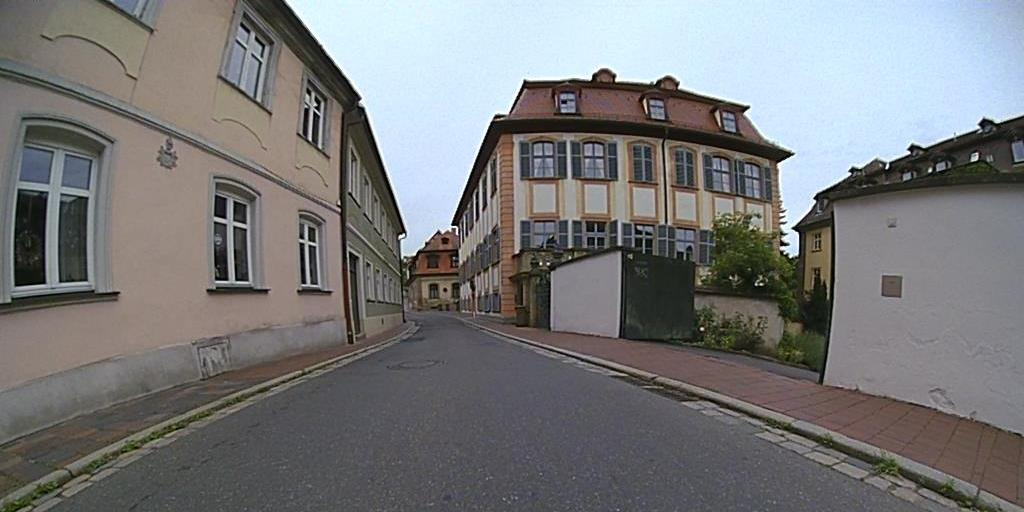} \\

{\rotatebox{90}{\hspace{0mm}\scriptsize}} &
\includegraphics[height=\turnheightnew]{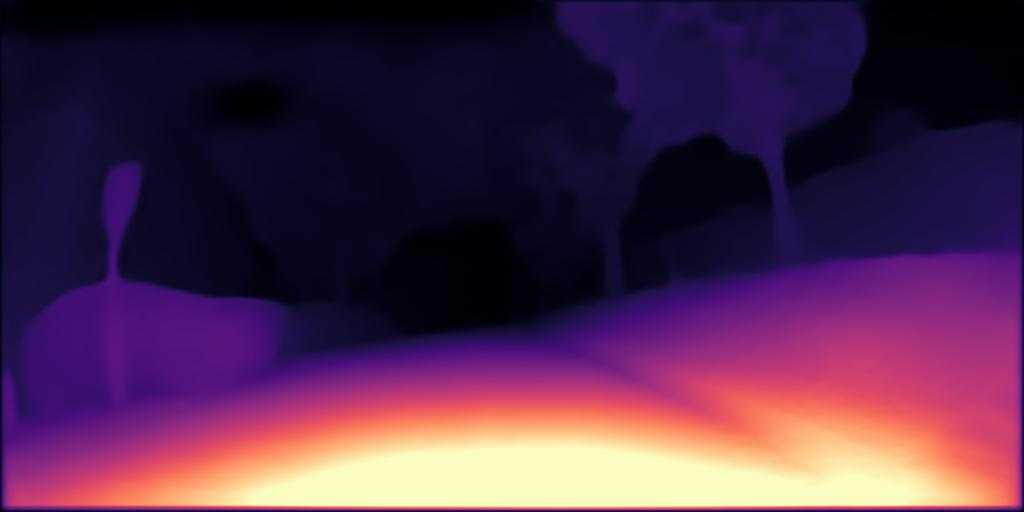} &
\includegraphics[height=\turnheightnew]{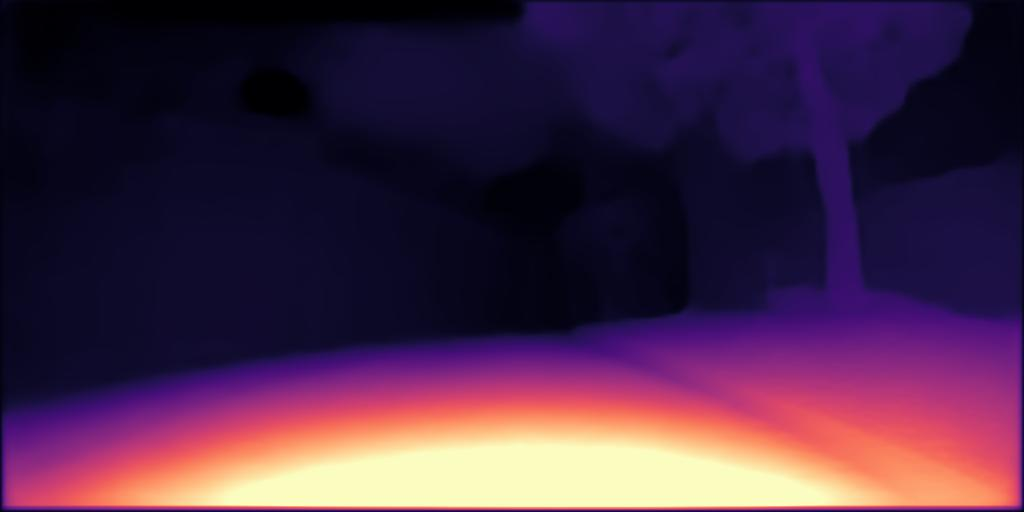} &
\includegraphics[height=\turnheightnew]{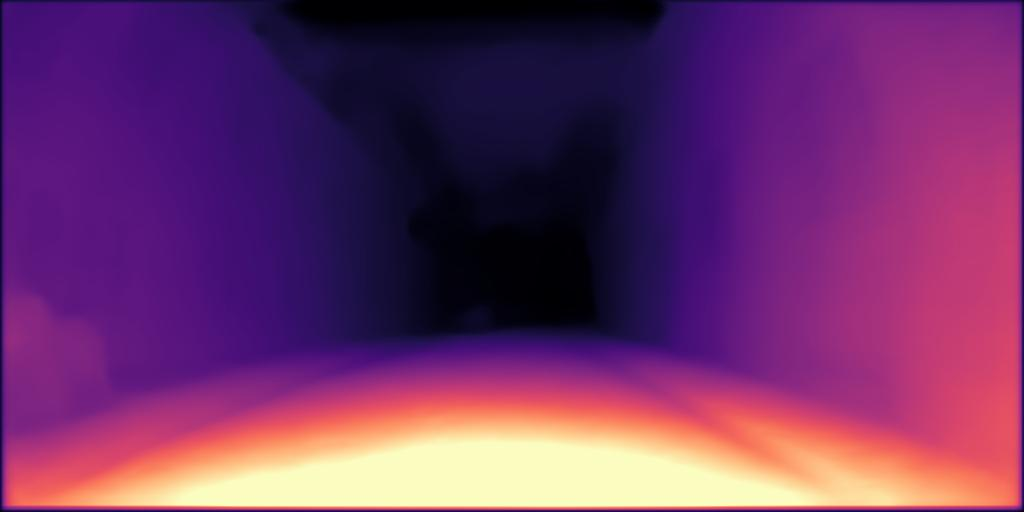} &
\includegraphics[height=\turnheightnew]{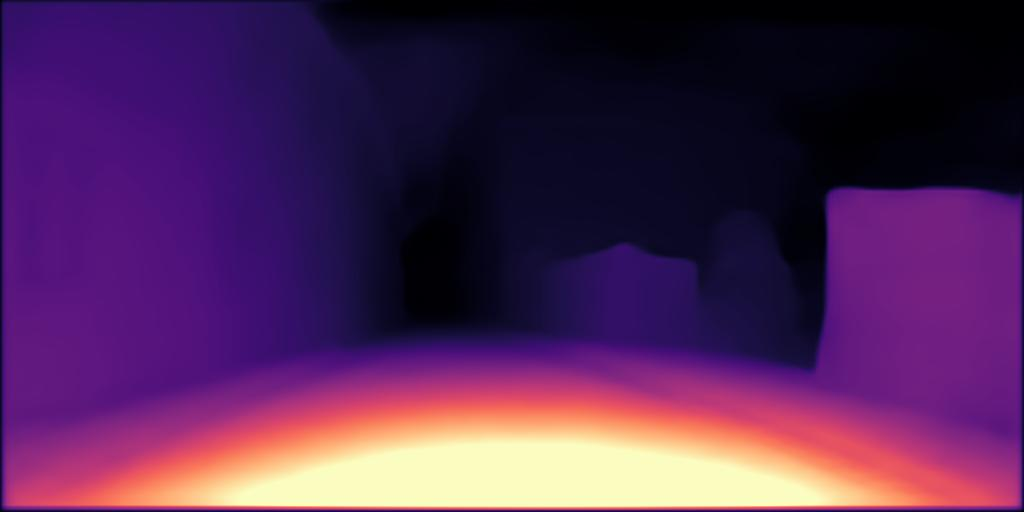} \\

% Tunnel
{\rotatebox{90}{\hspace{0mm}\scriptsize}} &
\includegraphics[height=\turnheightnew]{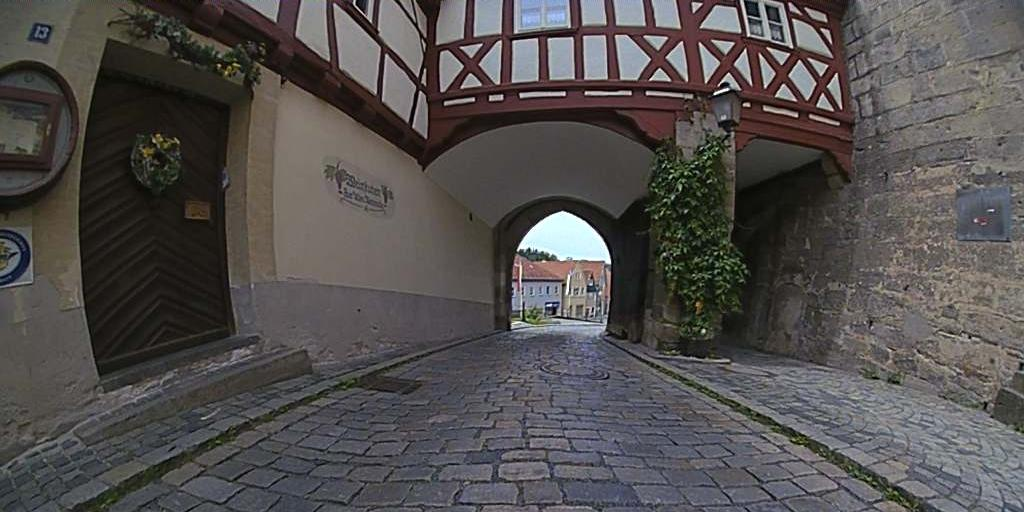} &
\includegraphics[height=\turnheightnew]{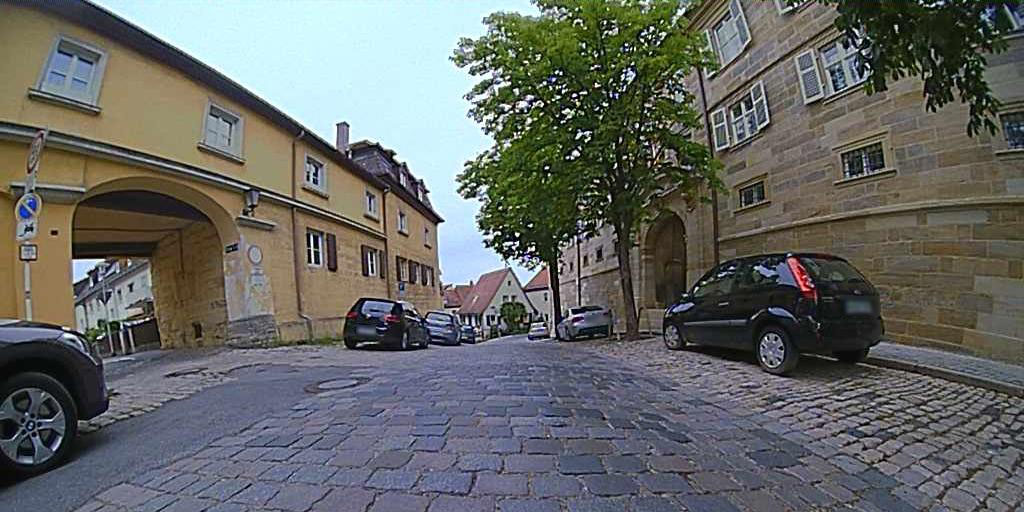} &
\includegraphics[height=\turnheightnew]{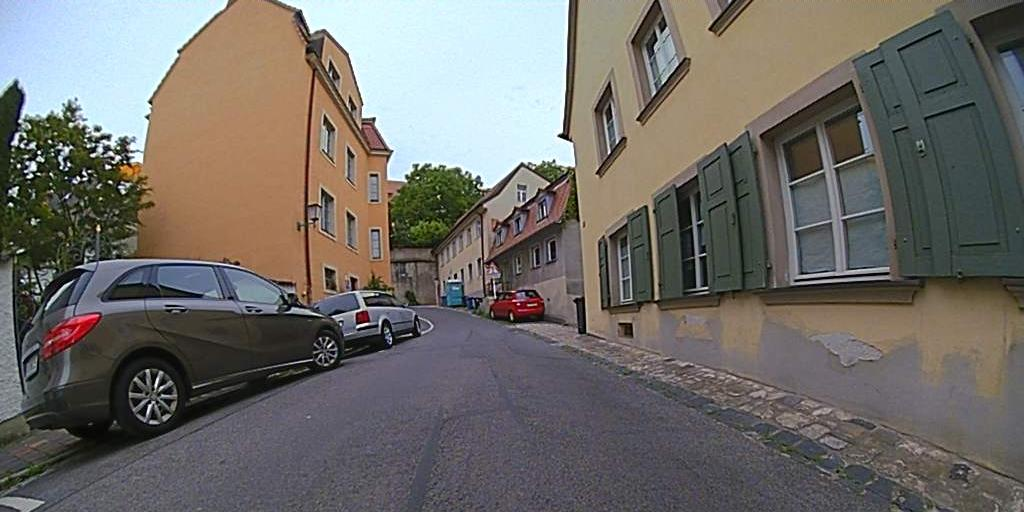} &
\includegraphics[height=\turnheightnew]{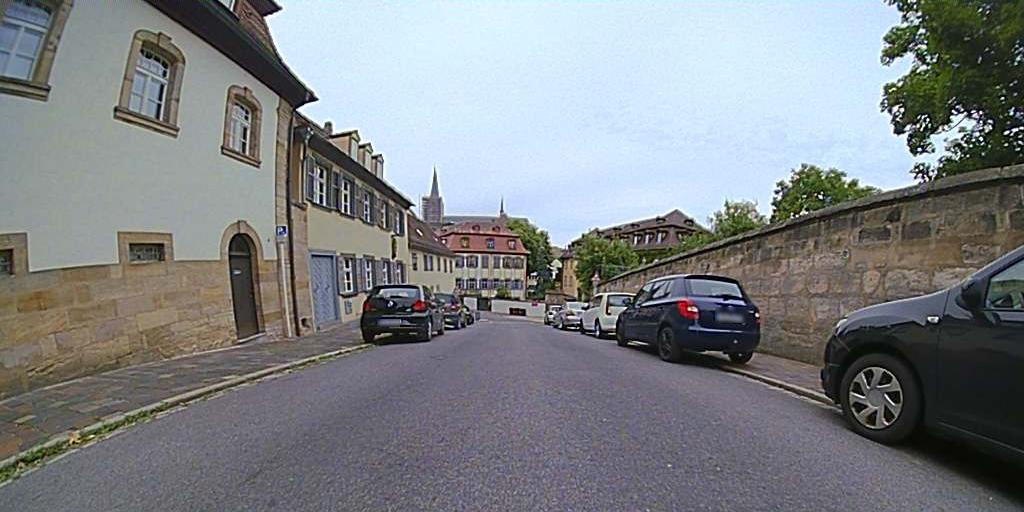} \\

{\rotatebox{90}{\hspace{0mm}\scriptsize}} &
\includegraphics[height=\turnheightnew]{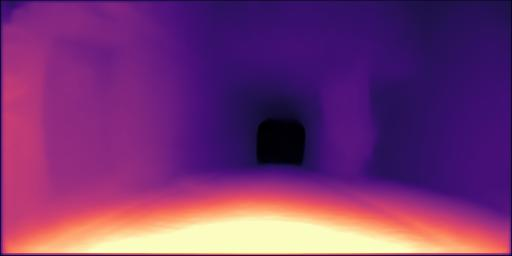} &
\includegraphics[height=\turnheightnew]{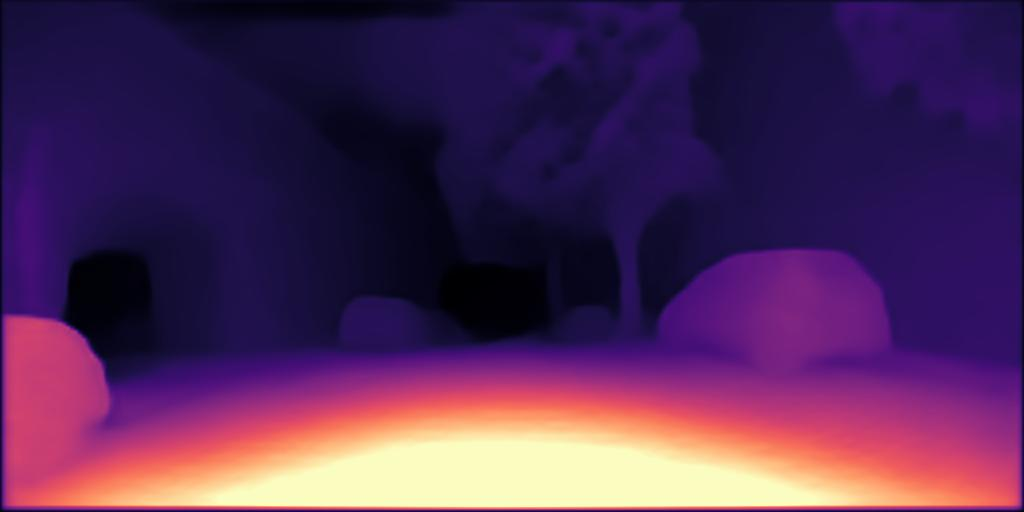} &
\includegraphics[height=\turnheightnew]{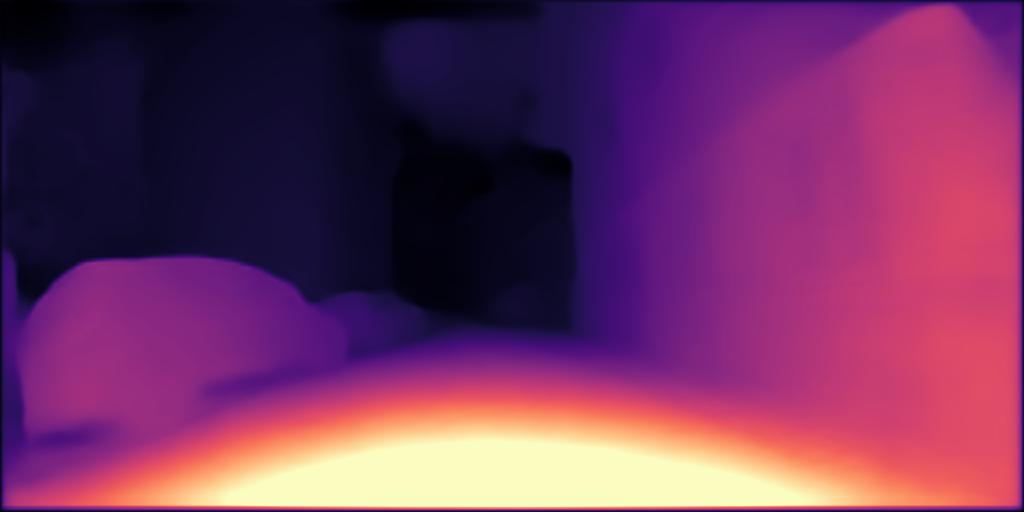} &
\includegraphics[height=\turnheightnew]{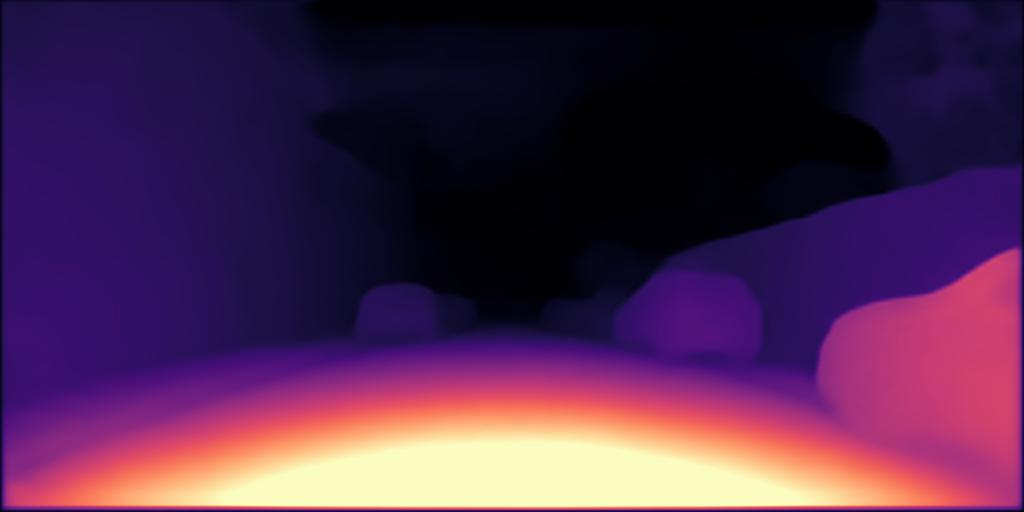} \\

%560 is left out
% Sharp
{\rotatebox{90}{\hspace{0mm}\scriptsize}} &
\includegraphics[height=\turnheightnew]{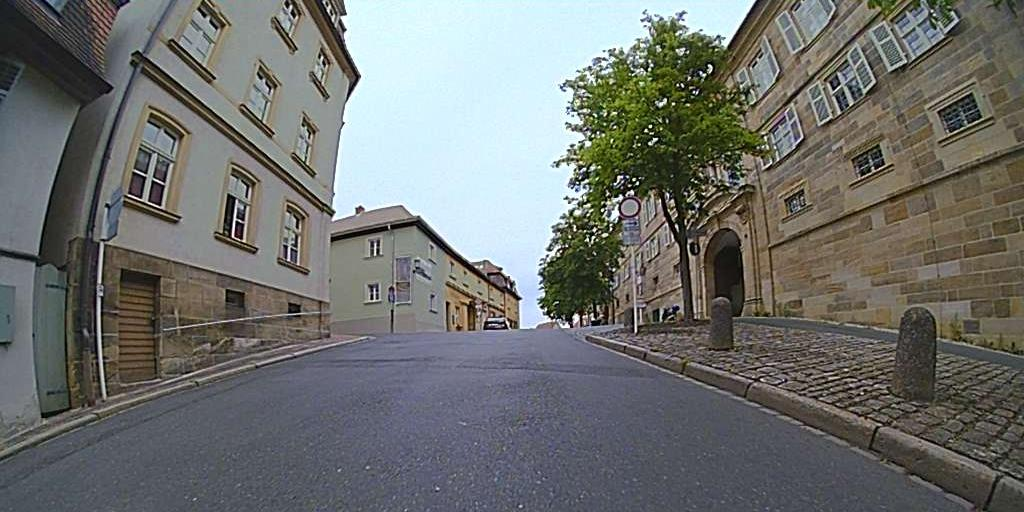} &
\includegraphics[height=\turnheightnew]{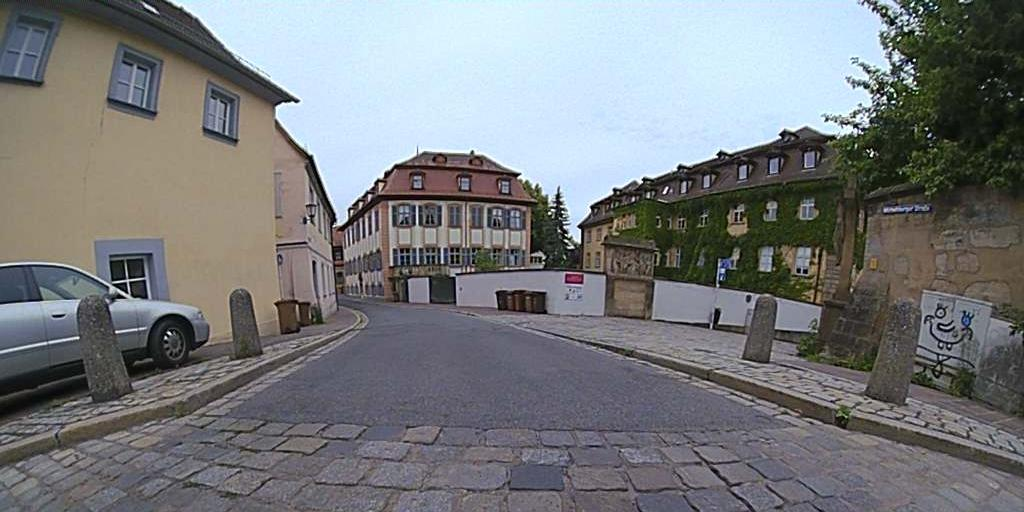} &
\includegraphics[height=\turnheightnew]{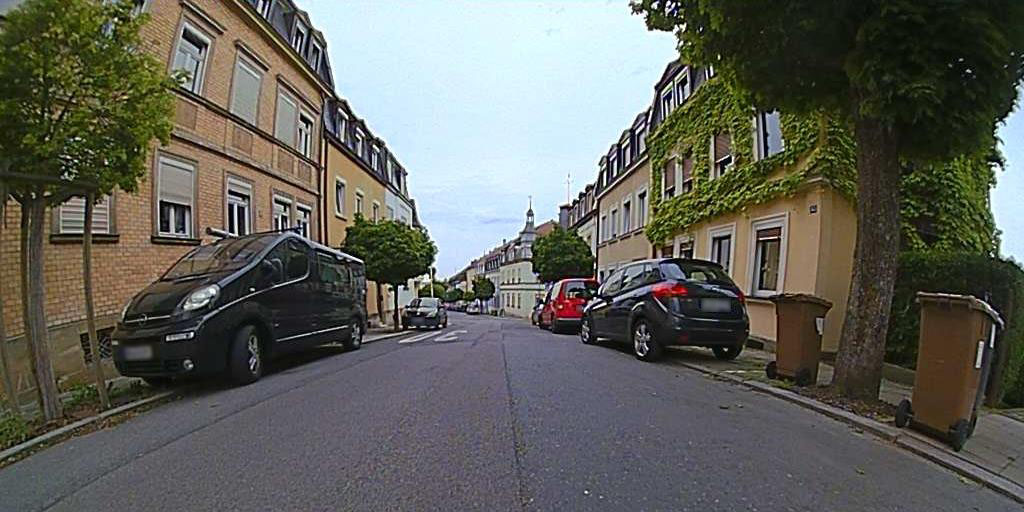} &
\includegraphics[height=\turnheightnew]{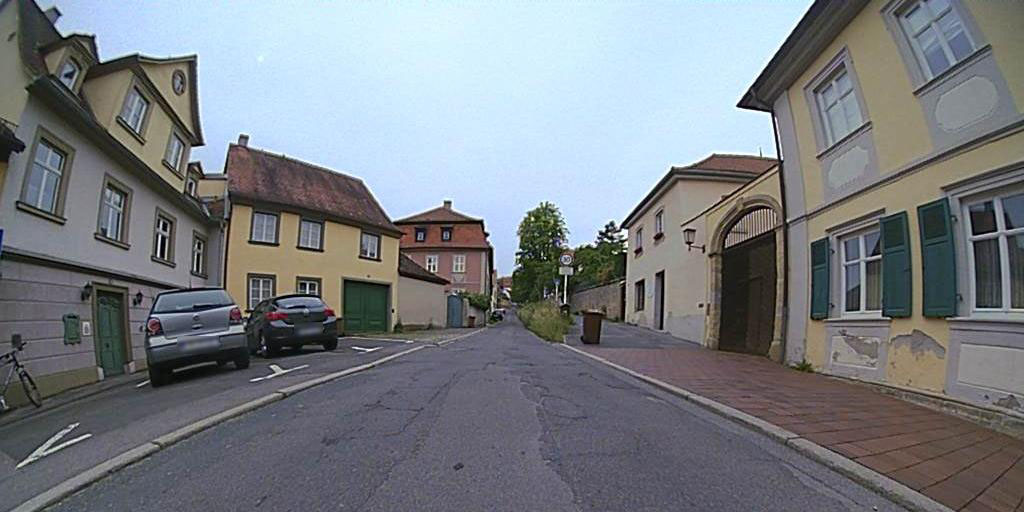} \\

{\rotatebox{90}{\hspace{0mm}\scriptsize}} &
\includegraphics[height=\turnheightnew]{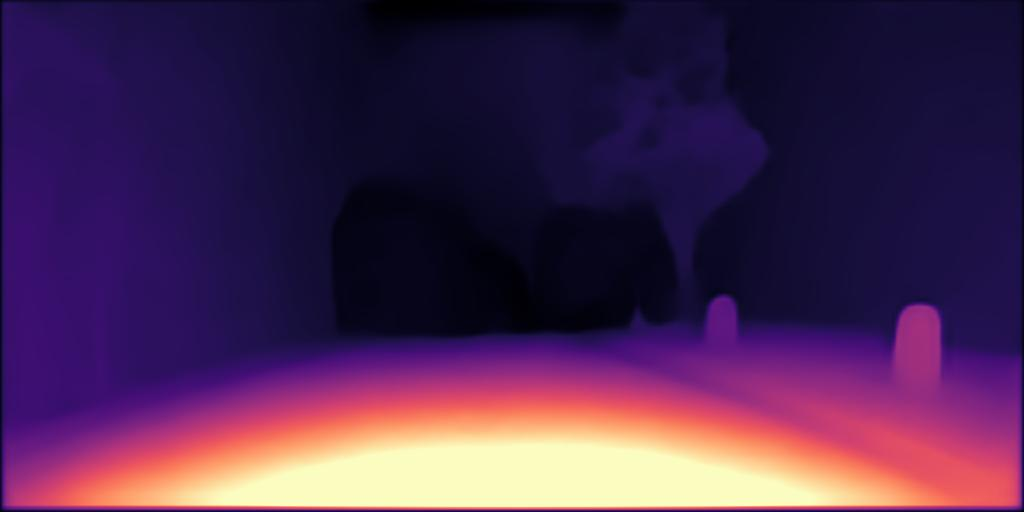} &
\includegraphics[height=\turnheightnew]{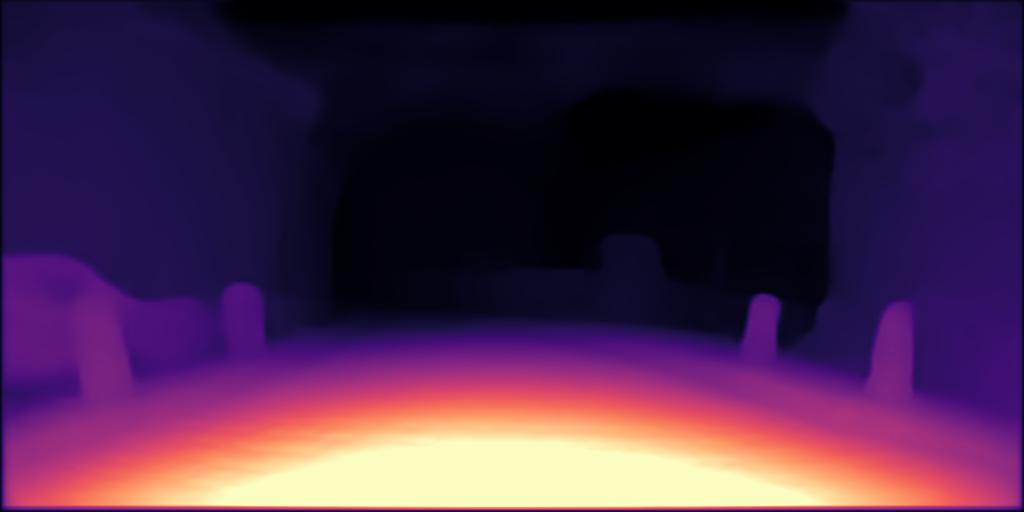} &
\includegraphics[height=\turnheightnew]{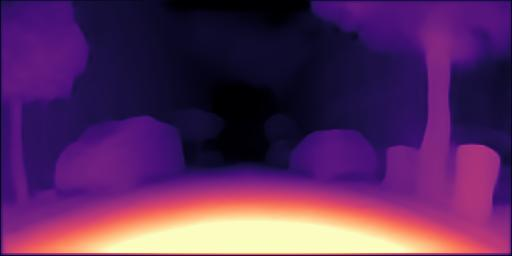} &
\includegraphics[height=\turnheightnew]{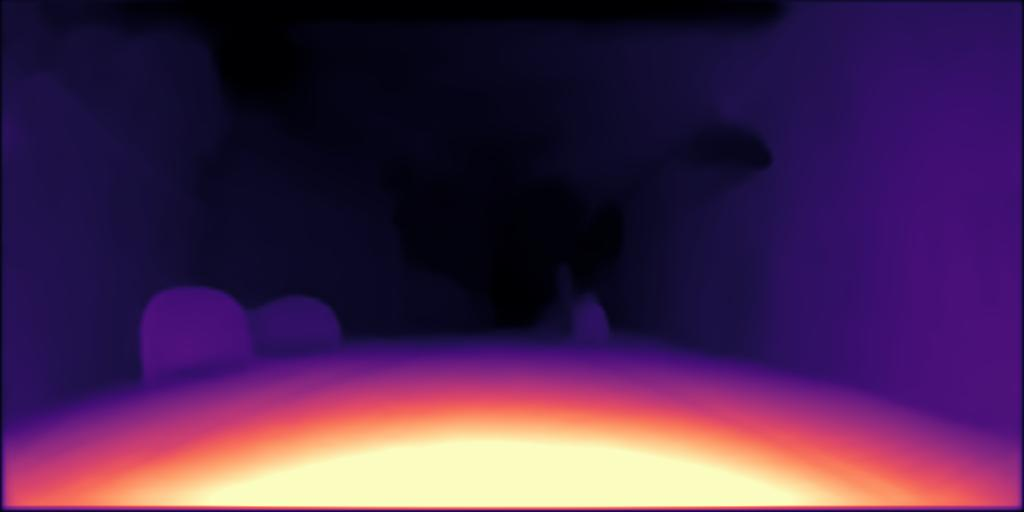} \\
\end{tabular}
}
  \caption{\textbf{Qualitative results on the Fisheye WoodScape~\cite{yogamani2019woodscape}}. In the 4th row of the table, we can see that our model adapts to the extreme distortion induced by the fisheye camera and produces sharp distance maps. In the 6th row, we can clearly see the sharp curbs on the street. Finally, in the last few rows, our model adapts to most of the complex scenes and produces very sharp scale-aware distance maps.}
  \label{fig:fisheye_suppl_qual}
\end{figure*}
% -------------------------------------------------
