# Supplementary material for: FisheyeDistanceNet: Self-Supervised Scale-Aware Distance Estimation using Monocular Fisheye Camera for Autonomous Driving
Source: arXiv:1910.04076 source file (2020-10-06)
Supplement: Supplementary file 2 [file related_work.tex]

\section{Related Work}

We aim to learn the task of dense distance estimation on raw fisheye images without any rectification. However, we are not aware of any previous work on specifically this task and therefore review learning based approaches for spherical content. Furthermore, we discuss recent monocular dense depth estimation methods for pinhole models.

\subsection{Learning for spherical images}

Plagemann et al.~\cite{plagemann2010nonparametric} proposed one of the earliest approaches using machine learning for estimating distances purely from spherical input by predicting over a range value per image rather than predicting the distance per pixel to drive robotic navigation.
However, modern ConvNets have dramatically changed the landscape of distance estimation. This enables us to apply spherical images to CNN framework by either directly on a projected (typically equirectangular) image, or by projecting the spherical content to the faces of a cube (cubemap) and running the CNN predictions on them, which are then merged by back-projecting them to the spherical domain. Ruder~\cite{ruder2018artistic} used cubemap projection, where each face was re-styled separately and then the cubemap was re-mapped back to the equirectangular domain for an artistic style transfer work. SalNet360's~\cite{monroy2018salnet360} saliency predictions on the cube’s faces are refined using their spherical coordinates and then merged back to $360^{\circ}$.

Given the difficulty to model the projection's distortion directly in typical CNNs as well as achieve invariance to the viewpoint's rotation, the alternative pursued by~\cite{frossard2017graph} is based on graph-based deep learning. Specifically they model distortion directly into the graph's structure and apply it to a classification task. In our previous work~\cite{varun18}, we trained distance estimation models in a supervised manner using sparse LIDAR data as ground truth. A novel approach taken in~\cite{su2017learning} is learning appropriate convolution weights for equirectangular projected spherical images by transferring them from an existing network trained on traditional 2D images. This conversion from the 2D to the $360^{\circ}$ domain is accomplished by enforcing consistency between the predictions of the 2D projected views and those in the $360^{\circ}$ image. Moreover, recent work on convolutions~\cite{jeon2017active,tateno2018distortion,dai2017deformable} that in addition to learning their weights also learn their shape, are very well suited for learning the distortion model of fisheye images, even though they have only been applied to fisheye lenses up to now by Deng et al.~\cite{deng2018restricted} for scene segmentation. However, these were only demonstrated in classification and single variable regression problems. In addition, they are also applied in the spectral domain while we formulate our network design for the spatial image domain.
% for distance estimation for fisheye camera

\subsection{Self-Supervised Monocular Depth and Pose estimation}

As supervised techniques for depth estimation advanced rapidly, the availability of target depth labels became challenging, especially for outdoor applications. To this end,~\cite{garg2016unsupervised,monodepth17} provided an alternative strategy involving training a monocular depth network with stereo cameras, without requiring ground-truth depth labels. By leveraging Spatial Transformer Networks~\cite{jaderberg2015spatial}, Godard et al~\cite{monodepth17} use stereo imagery to geometrically transform the right image plus a predicted depth of the left image into a synthesized left image. The loss between the resulting synthesized and original left images is then defined in a fully-differentiable manner, using a Structural Similarity~\cite{wang2004image} term and additional depth regularization terms, thus allowing the depth network to be self-supervised in an end-to-end fashion.

Following~\cite{monodepth17} and~\cite{ummenhofer2017demon}, Zhou et al.~\cite{zhou2017unsupervised} generalize this to self-supervised training in the \textit{purely} monocular setting, where a depth and pose network are simultaneously learned from unlabeled monocular videos. Several methods~\cite{yin2018geonet,mahjourian2018unsupervised,casser2019depth,zou2018df,klodt2018supervising,Wang_2018_CVPR,yang2018deep} have advanced this line of work by incorporating additional loss terms and constraints. All these methods, however, take advantage of constraints in monocular SfM that only allow the estimation of depth and pose up to an unknown scale factor on rectified images, and rely on the ground-truth LiDAR measurements to scale their depth estimates appropriately for evaluation purposes~\cite{zhou2017unsupervised}. 

In contrast to the approaches discussed above, we show that using view synthesis as the main supervisory signal along with deformable convolutions~\cite{dai2017deformable} and bolster from the car's instantaneous velocity during training, we are able to learn a \textit{scale-aware} distance and pose model on fisheye images, eliminating the impractical usage of LiDAR ground-truth distance measurements at inference-time.

% -------------------------------------------------
