# Supplementary material for: FisheyeDistanceNet: Self-Supervised Scale-Aware Distance Estimation using Monocular Fisheye Camera for Autonomous Driving
Source: arXiv:1910.04076 source file (2020-10-06)
Supplement: Supplementary file 3 [file supplementary.tex]

% -------------------------------------------------
% FAILURE CASES for Fisheye
\begin{figure*}[!ht]
  \captionsetup{singlelinecheck=false, justification=raggedright, font=footnotesize, labelsep=space}
  \centering
  \resizebox{\textwidth}{!}{
  \newcommand{\turnheightnew}{0.25\columnwidth}
\centering

\begin{tabular}{@{\hskip 0.5mm}c@{\hskip 0.5mm}c@{\hskip 0.5mm}c@{\hskip 0.5mm}c@{\hskip 0.5mm}c@{}}

{\rotatebox{90}{\hspace{0mm}}} &
\includegraphics[height=\turnheightnew]{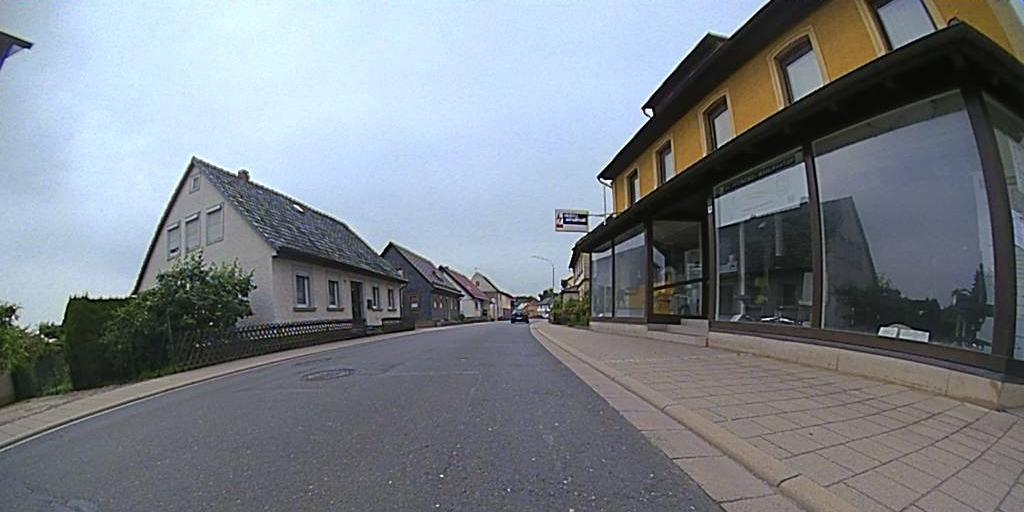} &
\includegraphics[height=\turnheightnew]{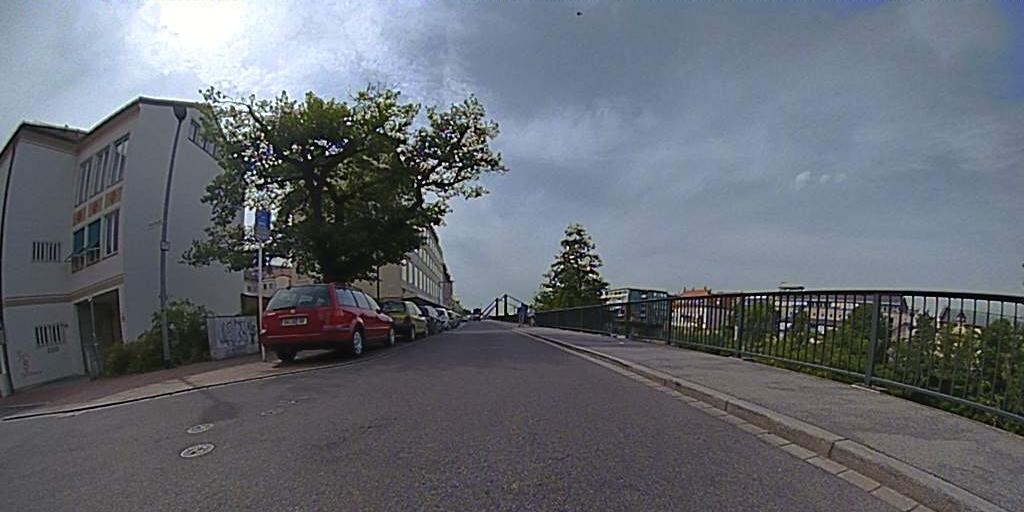} &
\includegraphics[height=\turnheightnew]{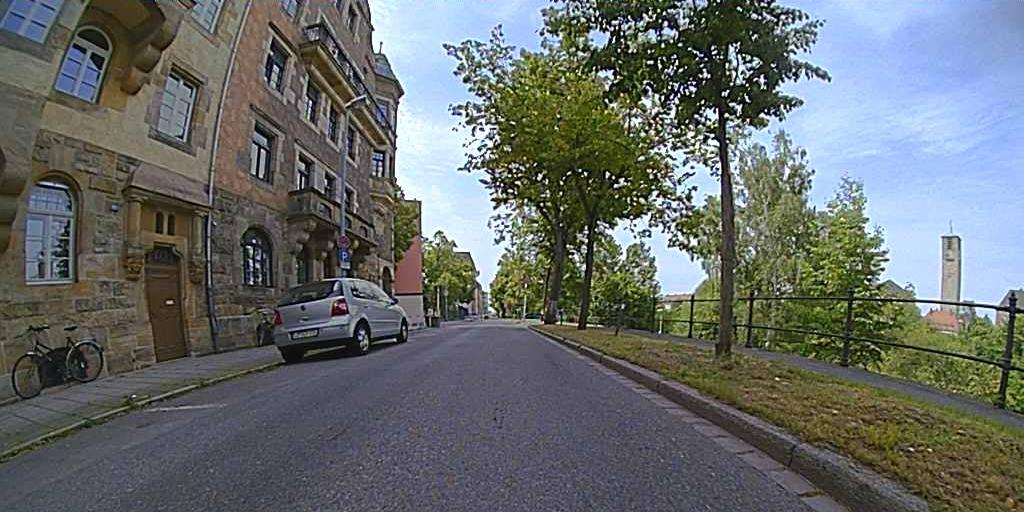} &
\includegraphics[height=\turnheightnew]{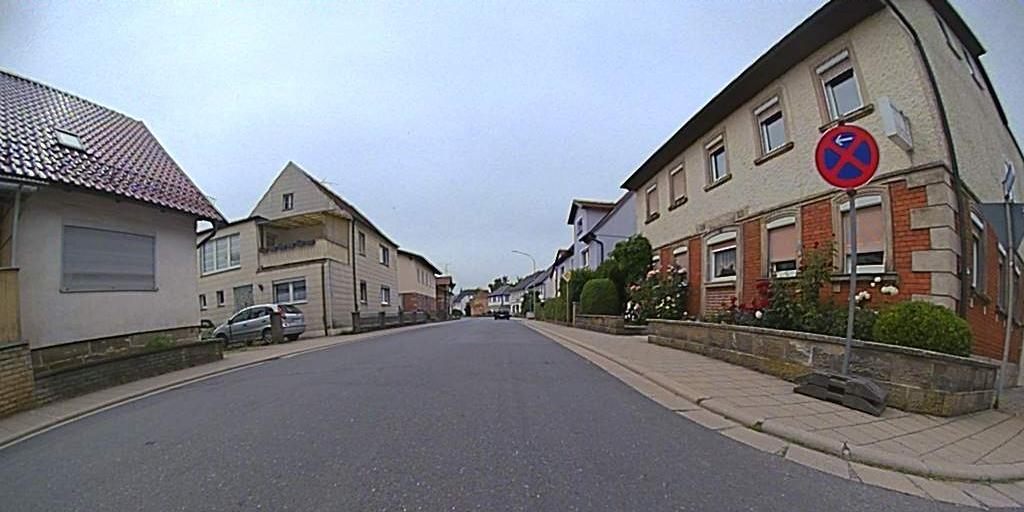}\\

{\rotatebox{90}{\hspace{0mm}\scriptsize}} &
\includegraphics[height=\turnheightnew]{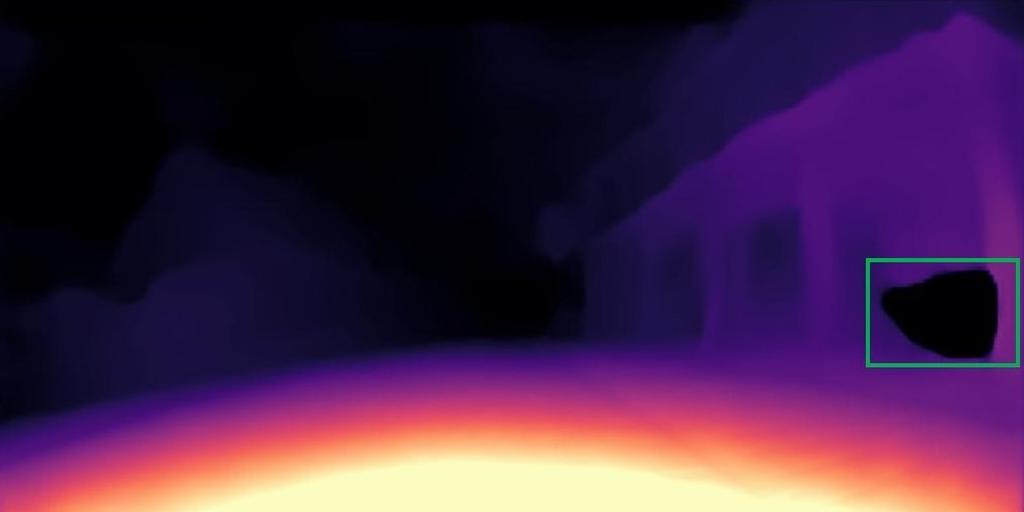} &
\includegraphics[height=\turnheightnew]{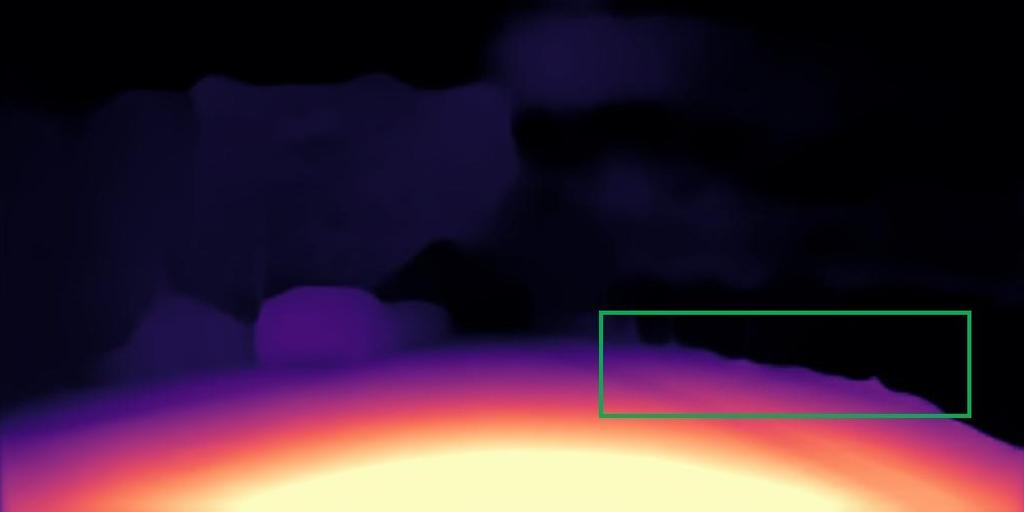} &
\includegraphics[height=\turnheightnew]{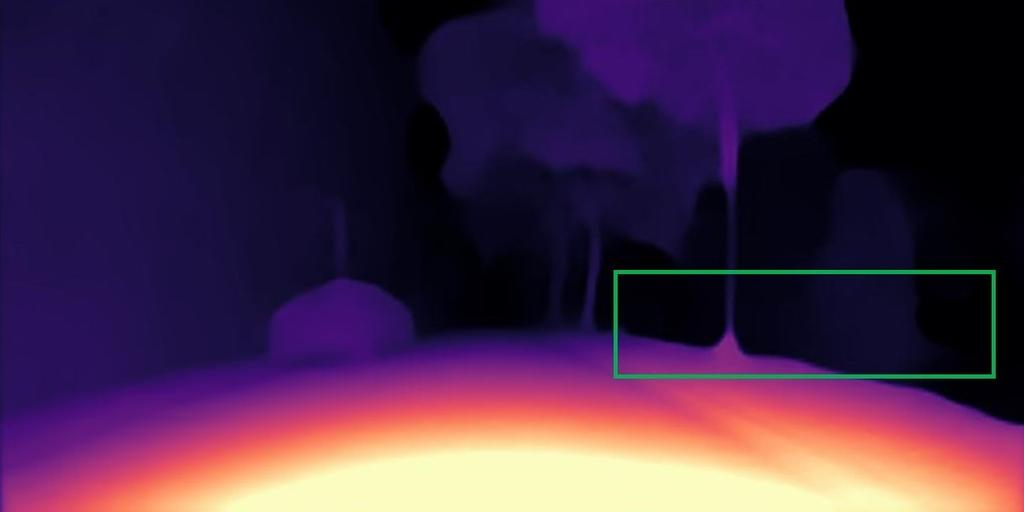} &
\includegraphics[height=\turnheightnew]{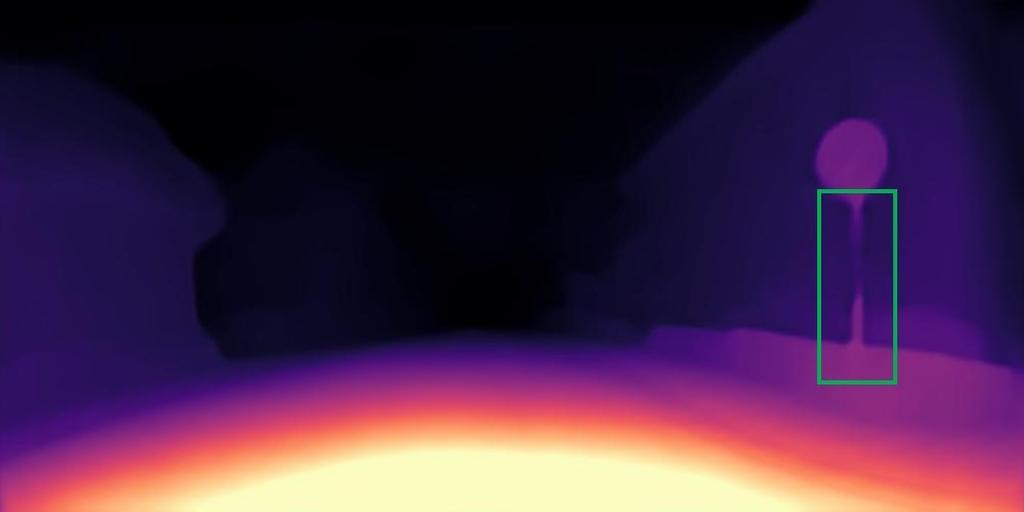} \\

\end{tabular}
}
  \caption{\textbf{Failure Cases on the Fisheye WoodScape~\cite{yogamani2019woodscape} dataset.}
  The photometric loss fails to learn good distances for reflective regions which can be seen in the $1^\text{st}$ figure. In the $2^\text{nd}$ and $3^\text{rd}$ figures shown above, the model fails to accurately delineate objects where boundaries are ambiguous.}
  \label{fig:fisheye_failure}
\end{figure*}

% -------------------------------------------------
% KITTI Ablation Quantitative table
\begin{table*}[t!]
\captionsetup{singlelinecheck=false, justification=raggedright, font=footnotesize, labelsep=space}
\small
\begin{center}
	\begin{tabular}{l|c|c|c|c|c|c|c|c|c|c|c}
	\hline
    Method & FS & BS & SR & CSDCL & Abs Rel & Sq Rel & RMSE & RMSE log & \cellcolor[HTML]{e8715b}$\delta < 1.25$ & \cellcolor[HTML]{e8715b}$\delta < 1.25^2$ &  \cellcolor[HTML]{e8715b}$\delta < 1.25^3$\\
    \hline\hline
    Ours & \checkmark & \checkmark & \checkmark & \checkmark & 0.117 & 0.867 & 4.739 & 0.190 & 0.869 & 0.960 & 0.982 \\
    Ours & \checkmark & \checkmark &            & \checkmark & 0.133 & 0.884 & 4.951 & 0.212 & 0.845 & 0.952 & 0.980 \\
    Ours & \checkmark &            &            & \checkmark & 0.134 & 0.929 & 5.063 & 0.215 & 0.835 & 0.947 & 0.979 \\
    Ours & \checkmark &            &            &            & 0.144 & 1.029 & 5.146 & 0.258 & 0.817 & 0.945 & 0.974 \\
    \hline
\end{tabular}
\end{center}
\caption{\textbf{Ablation study of our algorithm on the KITTI Eigen split dataset~\cite{geiger2013vision}}. Distances are capped at $80\,m$. BS, SR (ICNR), CSDCL, and DCN represent a backward sequence, super-resolution network with PixelShuffle, or sub-pixel convolution initialized to convolution NN resize (ICNR)~\cite{aitken2017checkerboard} and cross-sequence distance consistency loss, respectively. The input resolution is $640 \times 192$ pixels.}
\label{table:kittiablation}
\end{table*}
% -------------------------------------------------

\section{Limitation of normal 2D convolution}
\label{sec:limitation of 2d conv}

In a deep CNN, the upper layers encode high-level scene information with weak spatial information including object- or category-level evidence. Features from the middle layers are expected to describe middle-level representations of object parts and retain spatial information. Features from the lower convolution layers encode low-level spatial visual information like edges, corners, circles, etc. That means that the middle and lower layers are responsible for learning spatial structures. If the deformable convolution is applied to the lower or middle layers, the spatial structures are susceptible to fluctuation. The spatial correspondence between input images and output distance maps is difficult to be preserved. This is the spatial correspondence problem indicated in~\cite{li2017dense}, which is critical in pixel-wise distance estimation. Hence, deformable convolution is applied to the last few convolution layers as proposed by~\cite{dai2017deformable}.

To alleviate this problem, Zhu et al.~\cite{zhu2019deformable} proposed a better, more Deformable ConvNet with enhanced modeling power which can effectively model geometric transformations. We incorporate the enhanced modulated deformable convolutions to our \textit{FisheyeDistanceNet} and \textit{PoseNet}.

% -------------------------------------------------
\section{Depicting the importance of additional warps}
\label{sec:importance of warps}

In the forward sequence, we synthesize the target frame $I_t$ with the source frames $I_{t'}$ ($\ie$ as per the discussion in Section~\ref{sec:photometric loss} $t' \in \{t+1, \: t-1\}$). The reconstructed image $\hat{I}_{t' \to t}^{uv}$ will result in a zoom-in operation where the border distance values are useful and will get meaningful gradients to train with, but center values will have a lot of noise due to the low displacement. On the other hand since $\hat{I}_{t \to t'}^{uv}$ will result in a zoom-out effect, the border distance values are insignificant and should be filtered out from photo-metric loss because the pixel that has to be retrieved does not exist. Center distance though will have a warp that sample values from border of the frame, \ie with large displacement and the gradient will be less noisy than with $\hat{I}_{t' \to t}^{uv}$. Additional warps will induce more constraints to avoid overfitting and resolves unknown distances in the borders at the test time.

% -------------------------------------------------
\section{Further quantitative comparisons}
\label{sec:further quantitative comparison}

The quantitative results shown in the Table~\ref{tab:results} show that our scale-aware self-supervised approach outperforms all the state-of-the-art monocular approaches. More specifically, we outperform recent methods that explicitly compute motion masks (cp. EPC++~\cite{luo2018every}, Ranjan~\cite{ranjan2019competitive}, Godard~\cite{godard2018digging}). Due to a lack of odometry data on the Cityscapes, we could not leverage the dataset to benchmark our scale-aware framework. In contrast to PackNet-SfM~\cite{guizilini2019packnet}, which presumably uses a superior architecture compared to our super-resolution ResNet18, with capability of estimating scale-aware depths with their velocity supervision loss, we could achieve higher accuracy with subtle improvements to the standard ResNet18 and the training framework.

We could significantly achieve higher accuracy after 25 epochs compared to Pillai et al.~\cite{pillai2019superdepth} 1024$\times$384, PackNet-SfM's~\cite{guizilini2019packnet} 1280$\times$384 approach trained for 200 epochs. All previous monocular methods mentioned in the Table~\ref{tab:results} evaluate their depth predictions by scaling to the median ground-truth data from LiDAR as introduced by~\cite{zhou2017unsupervised}. We do not perform any per-image median scaling on the test set, our FisheyeDistanceNet outputs scale-aware depth estimates for pinhole models. Initially, an unscaled model is trained for several epochs. As the training progresses, scale-awareness is then induced into the framework.

% -------------------------------------------------
\section{KITTI Eigen Split Ablation Study}
\label{sec:kittieigenablation}

We conduct an ablation study to evaluate the importance of different components. We ablate the following components and report their impact on the distance evaluation metrics in Table~\ref{table:kittiablation}: 

\begin{enumerate}
    \item  \textit{Remove Backward Sequence}: The network is only trained for the forward sequence which consists of two warps as explained in Section~\ref{sec:backward sequence}.
    \item \textit{Additionally remove Super Resolution using sub-pixel convolution}: Removal of sub-pixel convolution has a minor impact on the pinhole model compared to dropping these layers in fisheye~\cite{yogamani2019woodscape}. Although, when compared to state-of-the-art method~\cite{godard2018digging} we could significantly achieve higher accuracy and resolve depths at longer distances accurately.
    \item \textit{Additionally remove cross-sequence distance consistency loss}: Removing the CSDCL mainly diminishes the baseline.
\end{enumerate}
% -------------------------------------------------
% FIG: KITTI Qualitative results
\begin{figure*}[!ht]
  \captionsetup{singlelinecheck=false, justification=raggedright, font=footnotesize, labelsep=space}
  \centering
  \resizebox{\textwidth}{!}{
  \newcommand{\turnheightnew}{0.195\columnwidth}
\centering

\begin{tabular}{@{\hskip 2mm}c@{\hskip 2mm}c@{\hskip 2mm}c@{\hskip 2mm}c@{\hskip 2mm}c@{}}

{\rotatebox{90}{\hspace{4mm}Input}} &
\includegraphics[height=\turnheightnew]{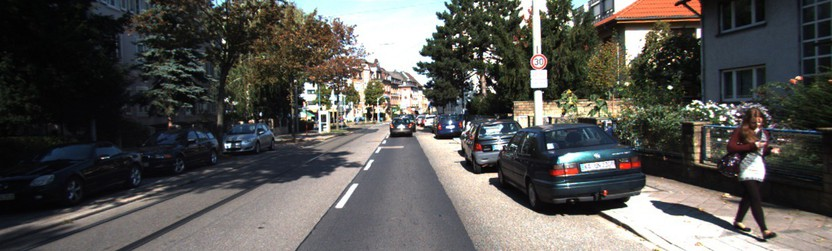} &
\includegraphics[height=\turnheightnew]{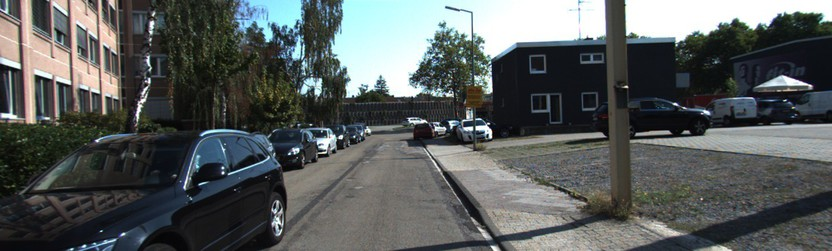} &
\includegraphics[height=\turnheightnew]{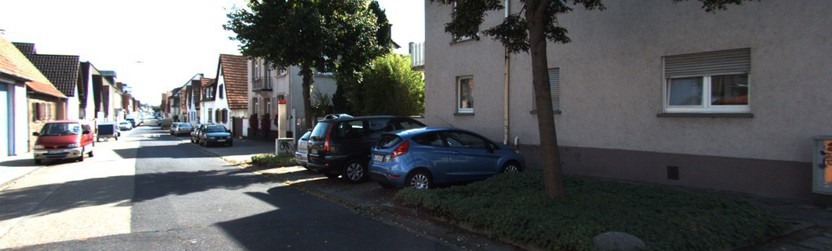} &
\includegraphics[height=\turnheightnew]{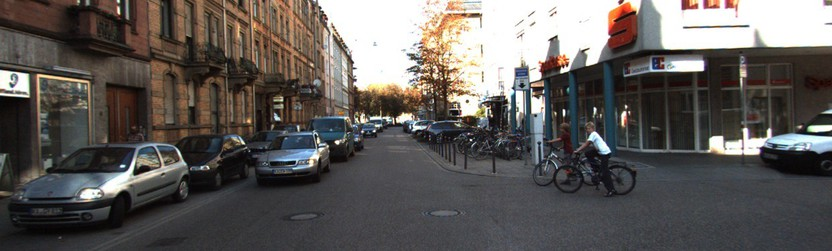}\\

{\rotatebox{90}{\hspace{0mm}\scriptsize
{Monodepth~\cite{monodepth17}}}} &
\includegraphics[height=\turnheightnew]{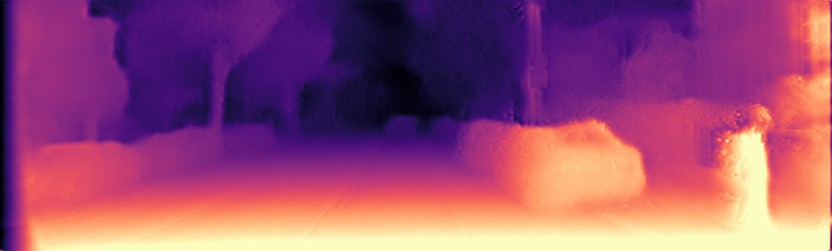} &
\includegraphics[height=\turnheightnew]{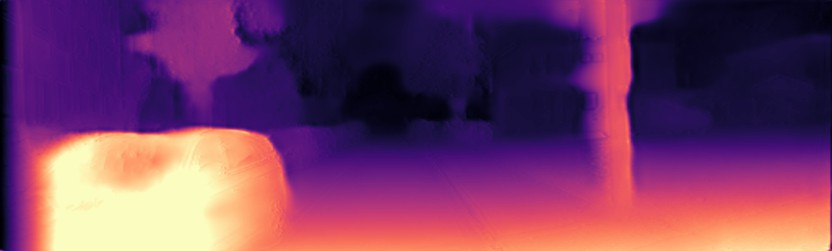} &
\includegraphics[height=\turnheightnew]{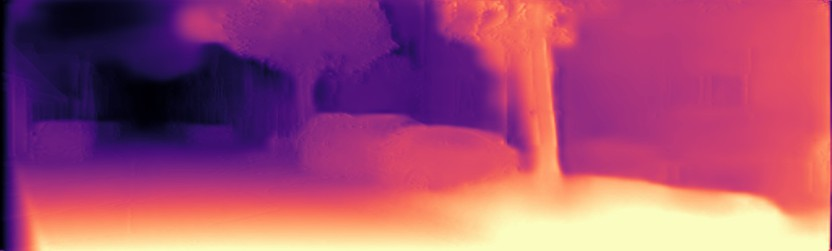} &
\includegraphics[height=\turnheightnew]{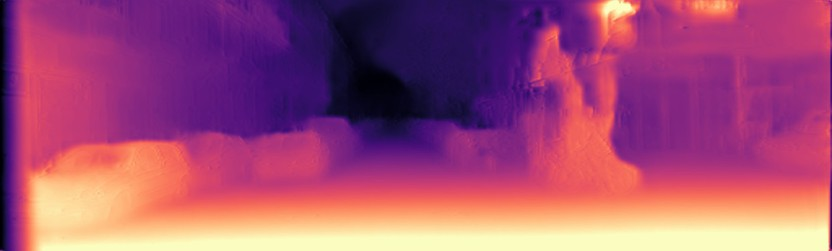} \\

{\rotatebox{90}{\hspace{0mm}\scriptsize
{Zhou et al.~\cite{zhou2017unsupervised}}}} &
\includegraphics[height=\turnheightnew]{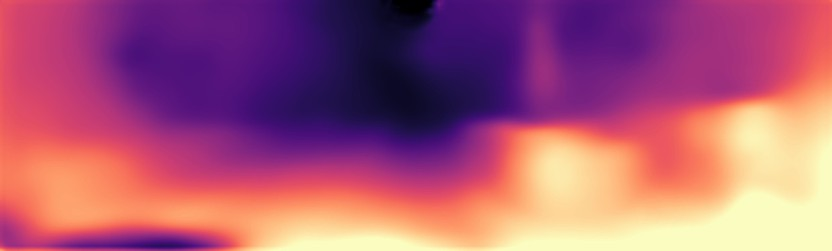} &
\includegraphics[height=\turnheightnew]{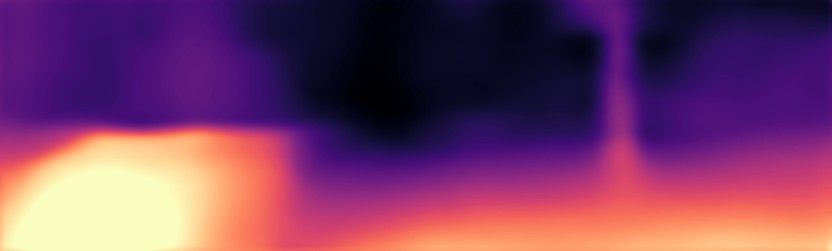} &
\includegraphics[height=\turnheightnew]{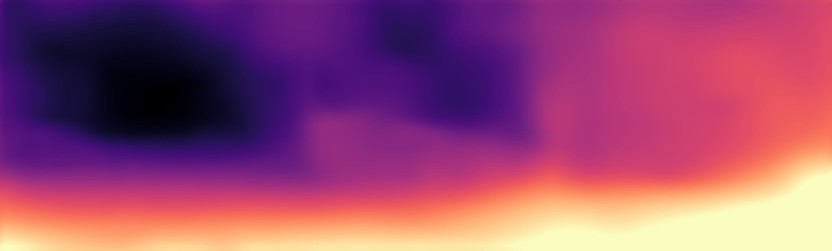} &
\includegraphics[height=\turnheightnew]{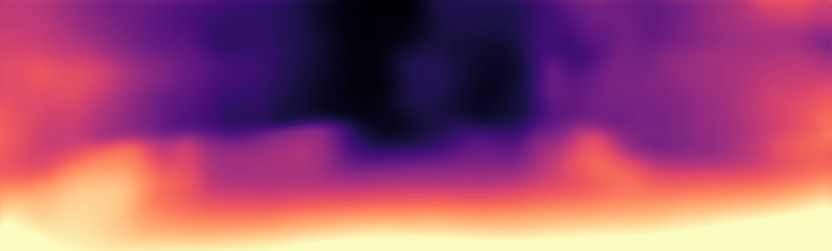} \\

{\rotatebox{90}{\hspace{2mm}\scriptsize
{DDVO~\cite{Wang_2018_CVPR}}}} &
\includegraphics[height=\turnheightnew]{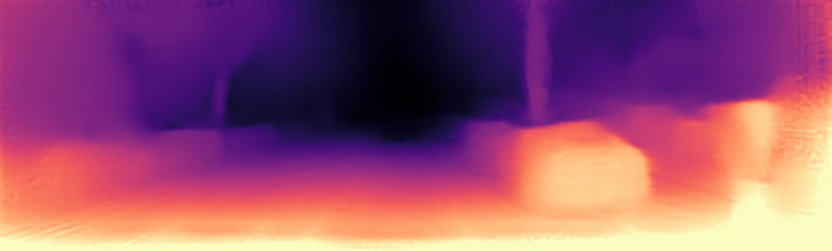} &
\includegraphics[height=\turnheightnew]{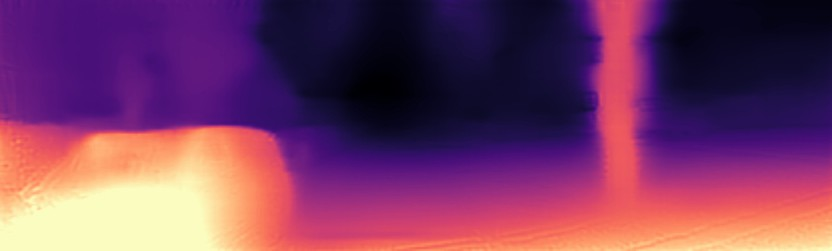} &
\includegraphics[height=\turnheightnew]{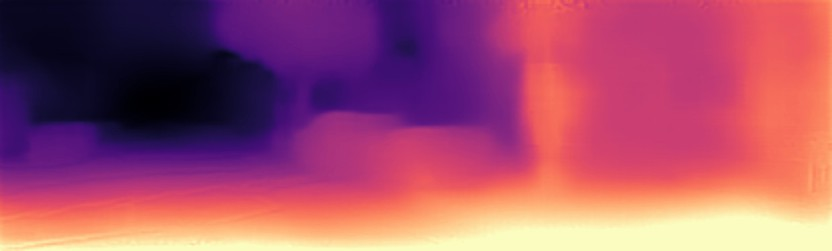} &
\includegraphics[height=\turnheightnew]{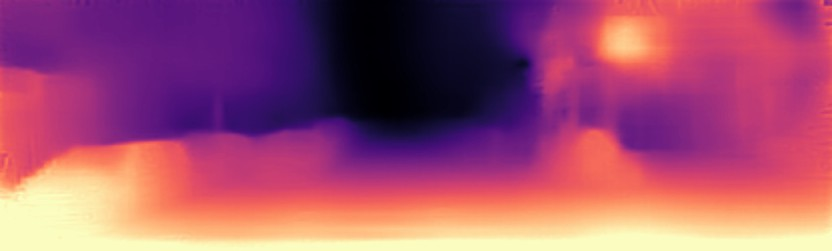} \\

{\rotatebox{90}{\hspace{2mm}\scriptsize
{GeoNet~\cite{yin2018geonet}}}} &
\includegraphics[height=\turnheightnew]{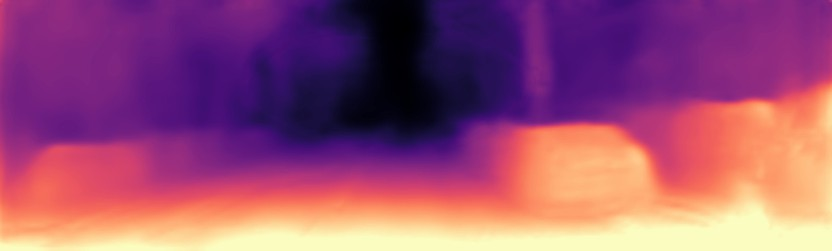} &
\includegraphics[height=\turnheightnew]{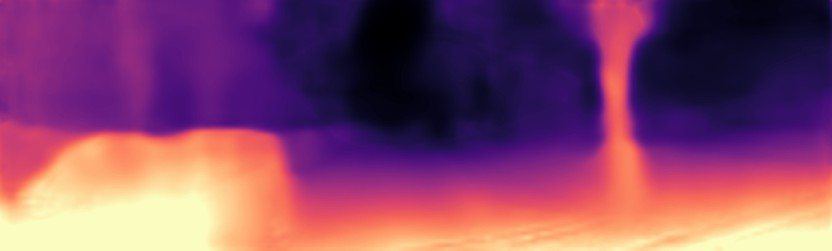} &
\includegraphics[height=\turnheightnew]{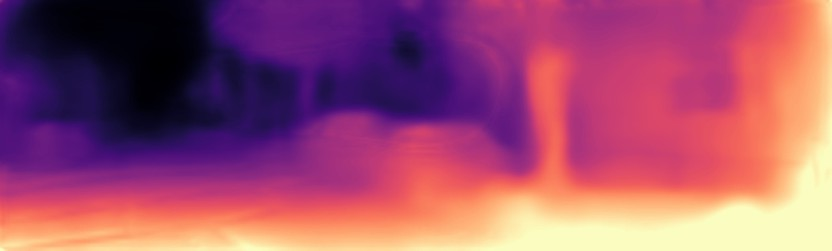} &
\includegraphics[height=\turnheightnew]{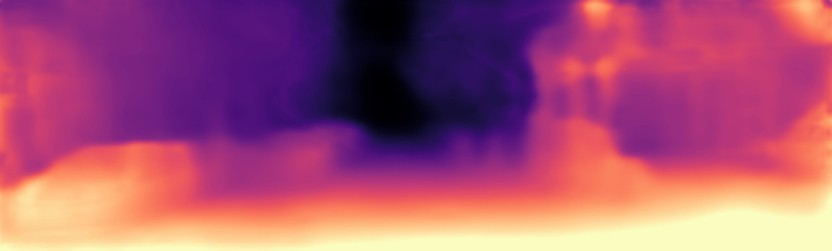} \\

{\rotatebox{90}{\hspace{0mm}\scriptsize
{Zhan et al.~\cite{zhan2018unsupervised}}}} &
\includegraphics[height=\turnheightnew]{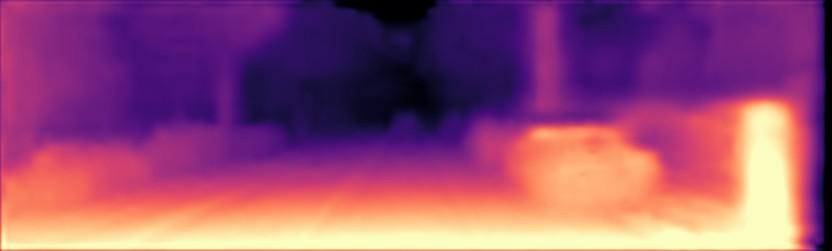} &
\includegraphics[height=\turnheightnew]{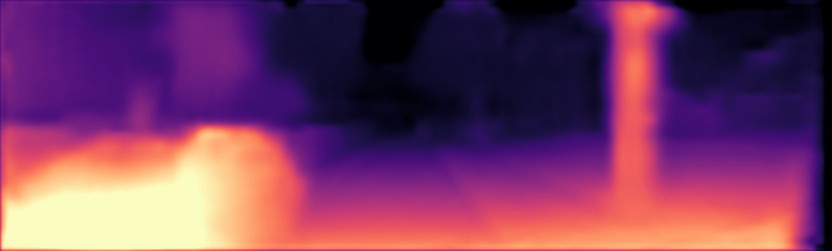} &
\includegraphics[height=\turnheightnew]{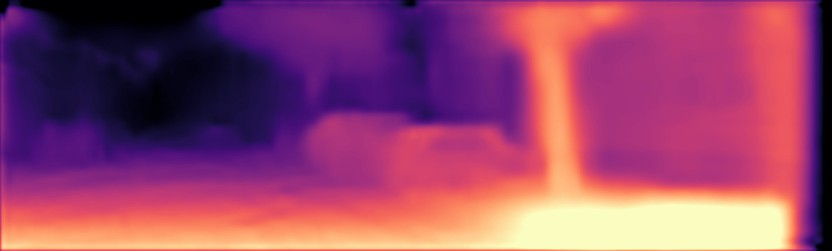} &
\includegraphics[height=\turnheightnew]{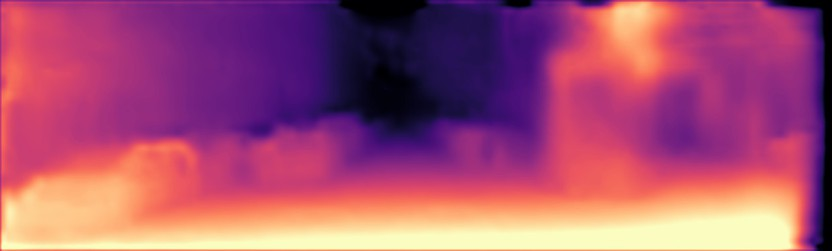} \\

{\rotatebox{90}{\hspace{-1mm}\scriptsize
Ranjan et al.~\cite{ranjan2019competitive}}} &
\includegraphics[height=\turnheightnew]{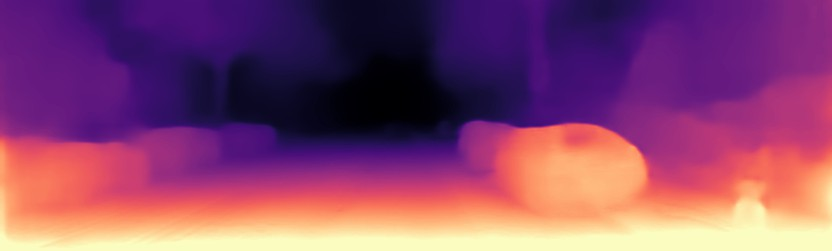} &
\includegraphics[height=\turnheightnew]{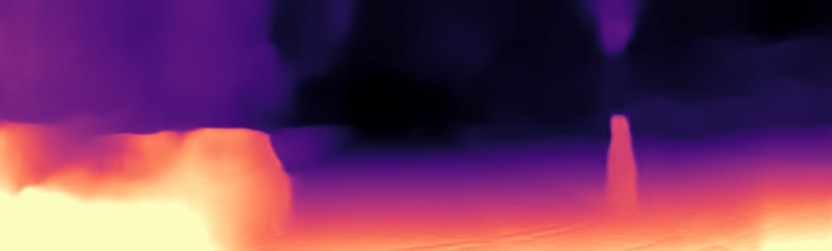} &
\includegraphics[height=\turnheightnew]{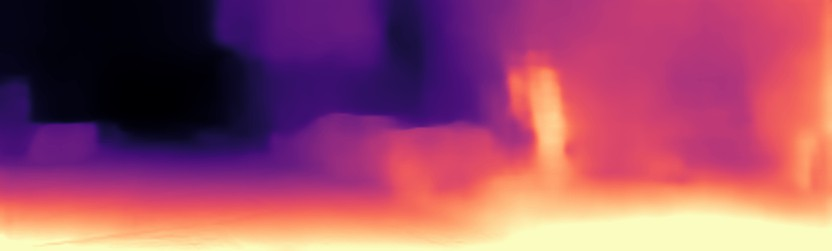} &
\includegraphics[height=\turnheightnew]{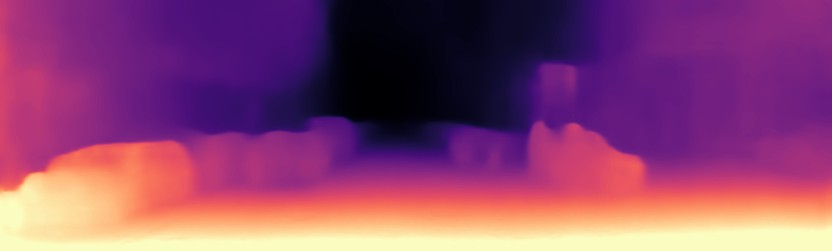} \\

{\rotatebox{90}{\hspace{0mm} \scriptsize
3Net-R50~\cite{luo2018every}}} &
\includegraphics[height=\turnheightnew]{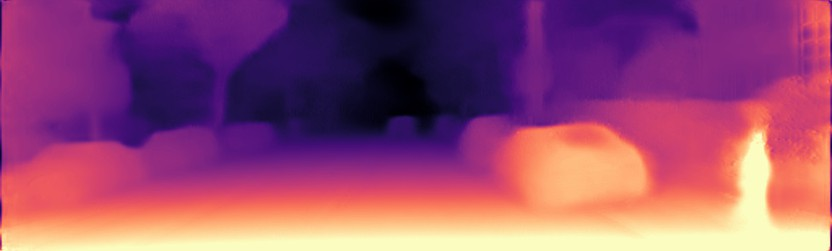} &
\includegraphics[height=\turnheightnew]{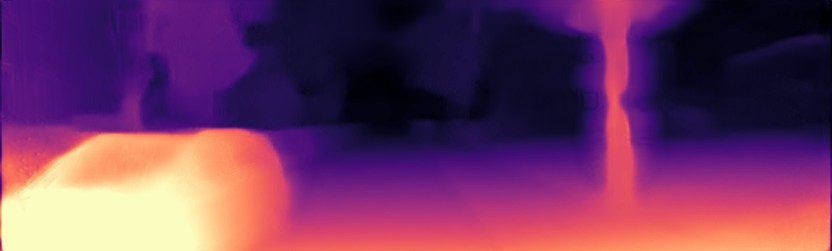} &
\includegraphics[height=\turnheightnew]{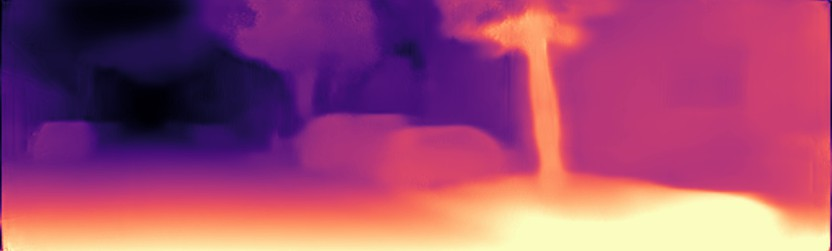} &
\includegraphics[height=\turnheightnew]{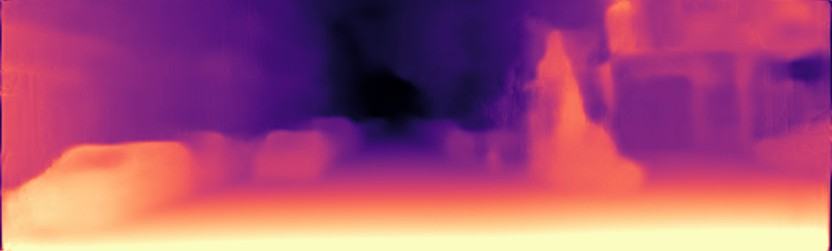} \\ 

{\rotatebox{90}{\hspace{0mm} \scriptsize
EPC++ (MS) \newline \cite{luo2018every}}} &
\includegraphics[height=\turnheightnew]{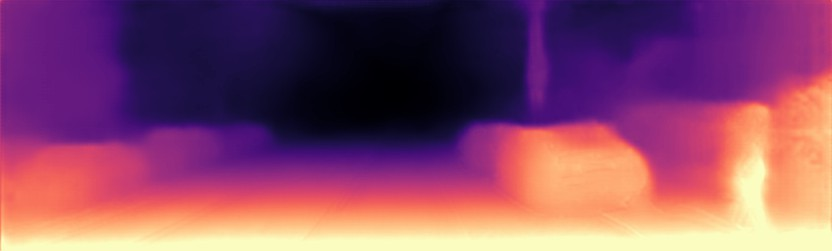} &
\includegraphics[height=\turnheightnew]{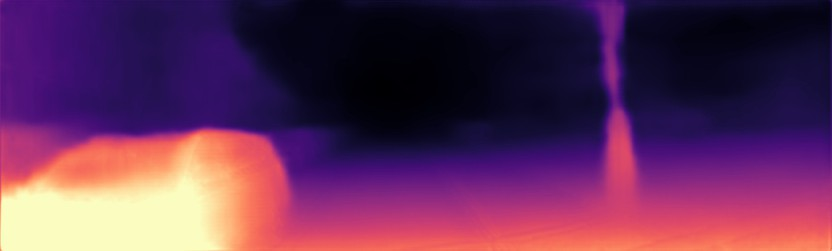} &
\includegraphics[height=\turnheightnew]{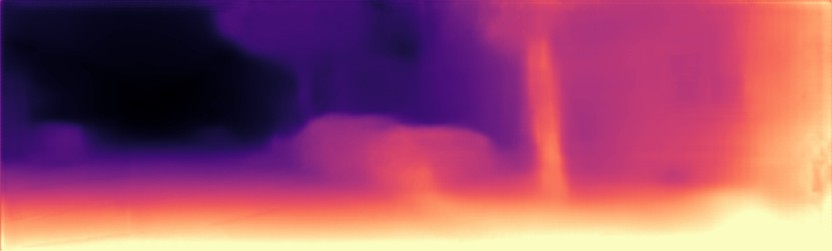} &
\includegraphics[height=\turnheightnew]{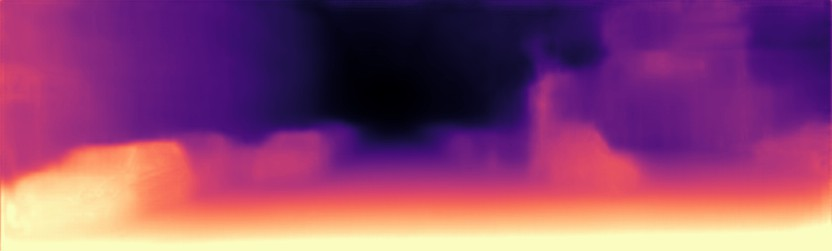} \\ 

{\rotatebox{90}{\hspace{0mm}\scriptsize
Monodepth2 M~\cite{godard2018digging}}} &
\includegraphics[height=\turnheightnew]{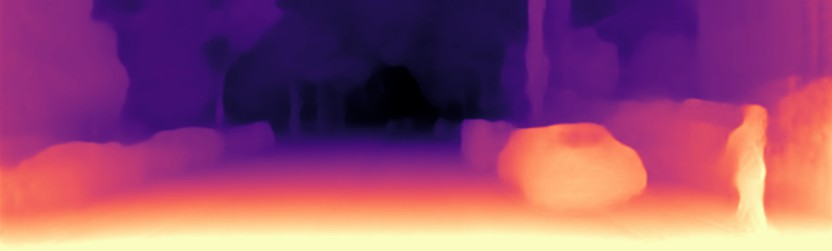} &
\includegraphics[height=\turnheightnew]{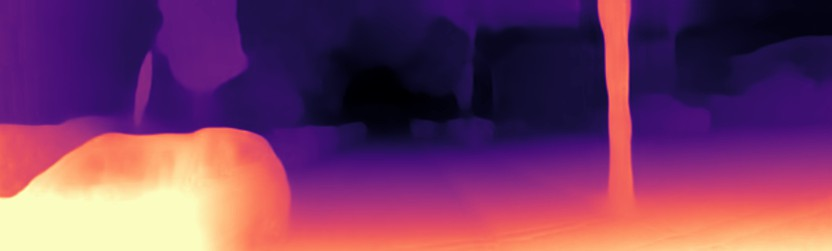} &
\includegraphics[height=\turnheightnew]{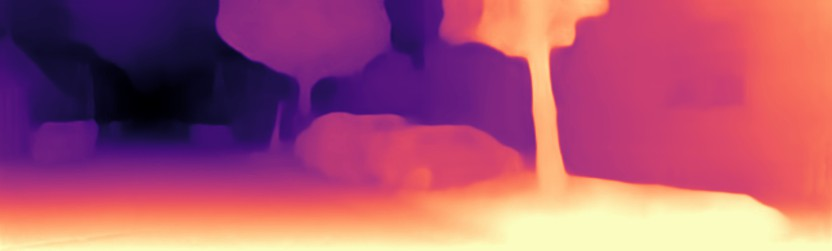} &
\includegraphics[height=\turnheightnew]{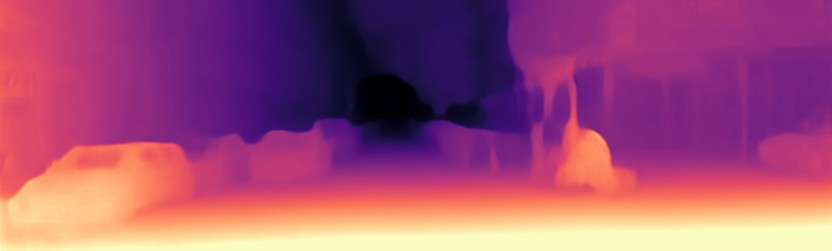} \\

{\rotatebox{90}{\hspace{3mm}\scriptsize
\textbf{Ours M}}} &
\includegraphics[height=\turnheightnew]{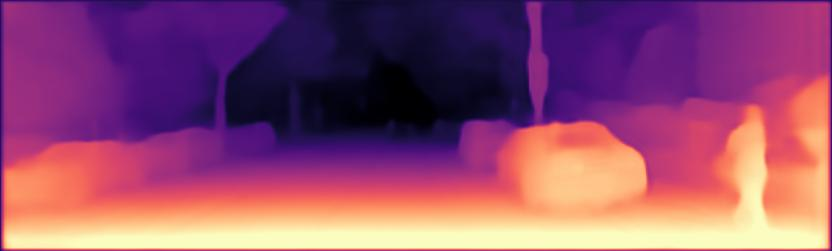} &
\includegraphics[height=\turnheightnew]{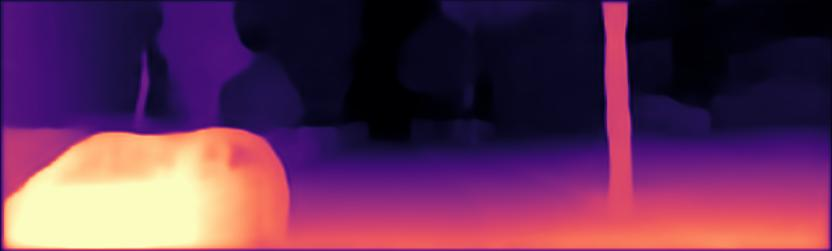} &
\includegraphics[height=\turnheightnew]{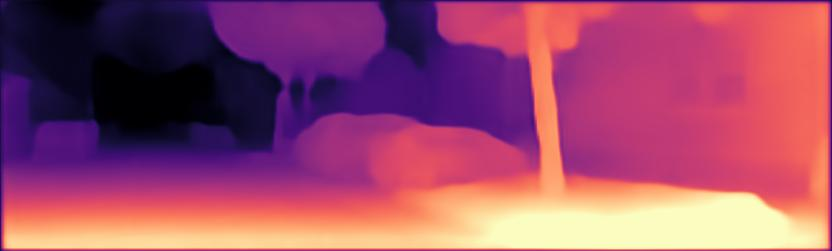} &
\includegraphics[height=\turnheightnew]{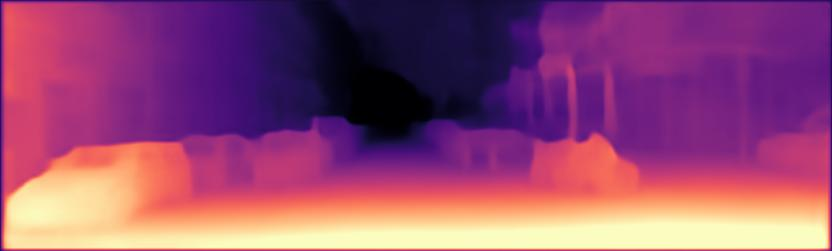} \\

\end{tabular}
}
  \caption{\textbf{Qualitative results on the KITTI Eigen split.} The qualitative table is taken from~\cite{godard2018digging} for a fair comparison, as our results produce similar sharp depth maps. When compared to Monodepth2 M~\cite{godard2018digging}, our model resolves the low textured areas such as sky i.e. infinite depth and provides sharper transition in the boundaries of objects. Our model (M) in the last row yields superior quantitative results which are reflected in Table~\ref{tab:results}.}
  \label{fig:kitti_eigen_qual}
\end{figure*}

% -------------------------------------------------
